# Supplementary material for: A Multimodal Corpus for Emotion Recognition in Sarcasm
Source: arXiv:2206.02119 source file (2022-06-05)
Supplement: Supplementary file 1 [file appendix.tex]

\section{Additional Analysis }\label{'sec:additional_analysis'}

\begin{table}[ht!]
\centering
% \resizebox{\columnwidth}{!}{%
\begin{tabular}{|r|c|c|c|c|c|c|}
\hline
\multicolumn{1}{|c|}{} & \multicolumn{1}{l|}{\textbf{An}} & \multicolumn{1}{l|}{\textbf{Sa}} & \textbf{Fr} & \textbf{Ri} & \textbf{Di} &\cellcolor{lightgray} \textbf{Total} \\ \cline{1-7} 
\textbf{PRO} & 47 & 15 & 61 & 129 & 81 & \cellcolor{lightgray}333 \\
\textbf{ILL} & 26 & 4  & 48 & 70  & 30 & \cellcolor{lightgray}178 \\
\textbf{EMB} & 13 & 5  & 20 & 27  & 22 &\cellcolor{lightgray} 87 \\
\textbf{LIK} & 1  & 0  & 1  & 0   & 1 & \cellcolor{lightgray}3  \\ \hline
\end{tabular}%

% }
% \captionsetup{justification=centering}
\caption{Implicit Emotion Distribution per Sarcasm Type. \footnotesize \{An-Anger, Sa-Sad, Fs-Frustrated, Dis-Disgust, Ri-Ridicule\} and \{PRO-Propositional, ILL-Illocutionary, EMB-Embedded, LIK-Likeprefixed\}}
\label{tab:emotion in sar-type}
\end{table}

\begin{table}[!h]
\centering
\resizebox{\columnwidth}{!}{%
\begin{tabular}{|c|c|c|c|c|c|c|c|c|c|c|}
\hline
                 & \textbf{An} & \textbf{Ex} & \textbf{Fe} & \textbf{Sa} & \textbf{Sp} & \textbf{Fs} & \textbf{Hp} & \textbf{Neu} & \textbf{Dis} & \textbf{Ri} \\ \hline
\textbf{Valence} & -0.5        & 0.6         & -0.7        & -0.9        & 0.05        & -0.5        & 0.95        & 0.0          & -0.8         & -0.55       \\
\textbf{Arousal} & 0.9         & 0.8         & 0.7         & -0.4        & 0.9         & 0.4         & 0.15        & 0.0          & 0.5          & 0.65        \\ \hline
\end{tabular}%
}
% \captionsetup{justification=centering}
\caption{Emotion wise Valence-Arousal Values present in new annotation,\scriptsize \{An-Anger, Ex- Excitement, Fe-Fear, Sa-Sad, Sp-Surprise, Fs-Frustrated, Hp-Happy Neu-Neutral, Dis-Disgust, Ri-Ridicule\}}
\label{tab:val-aro}
\end{table}

%%%%%%%%%%% Valence Arousal %%%%%%%%%%%
% Figure \ref{fig:val-aro} plots the valence and arousal values observed with different emotions in sarcastic sentences. Table \ref{tab:val-aro} shows the valence-arousal values with which the proposed dataset is annotated

\begin{figure}[h!]
\centering
        \includegraphics[totalheight=7cm]{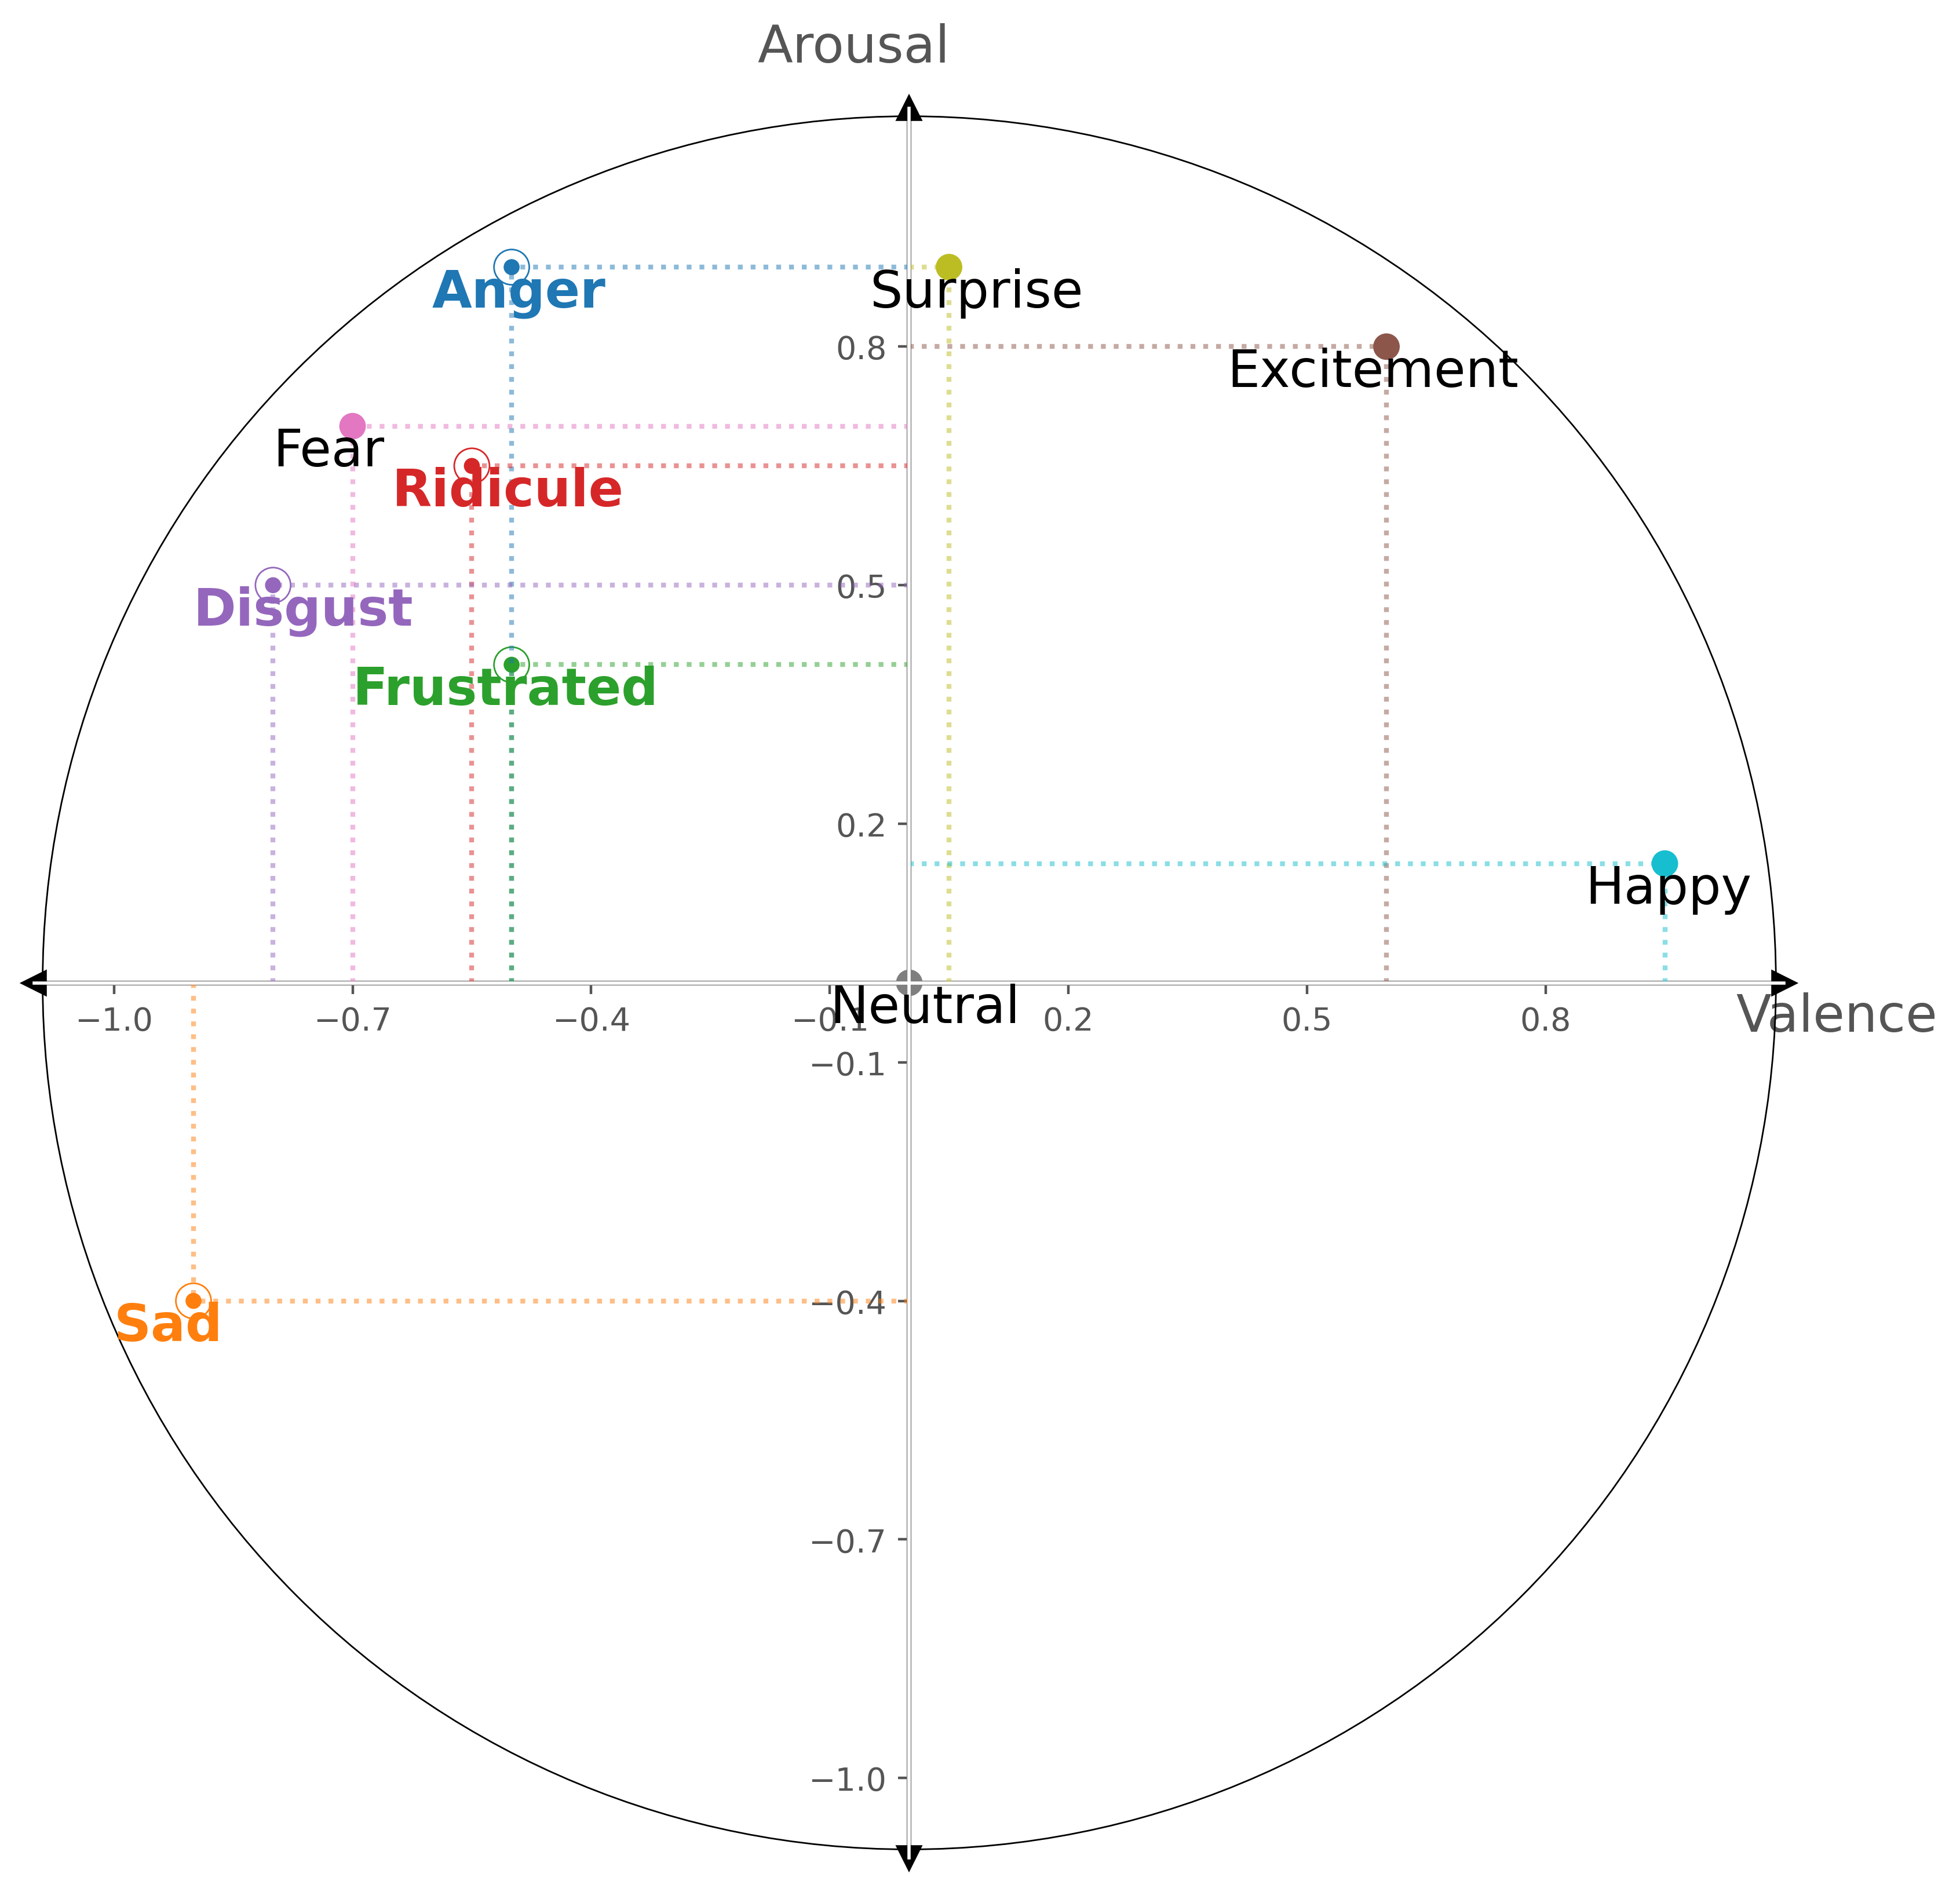}
    \captionsetup{justification=centering}
    \caption{Valence-Arousal Prediction\\ points with double circle are those which are present in sarcastic sentences}
    \label{fig:val-aro}
\end{figure}

%%%%%%%%%%% Prosodic %%%%%%%%%%%
Attention over modalities showed that for explicit emotion, text modality got highest weights whereas for implicit emotions video modality got higher weight over text. Audio modality has been equally important for implicit and explicit emotions. Intra-modality attention over audio features show relative importance of MFCC, spectrogram and prosodic features wherein within prosodic features we could clearly see importance of certain markers. Prosodic feature have 4 major components:  fundamental frequency (f0), voicing, harmonics-to-noise ration (HNR), and Loudness. For example: While loudness gets highest attention for anger and excitement emotions, prosodic features don't contribute at all to neutral emotion.

Figure \ref{fig:prosodic} represents the analysis on prosodic feature.
\begin{figure}[ht!]
\centering
    %     \includegraphics[totalheight=3.3cm]{img/prosodic.png}
    % \caption{Prosodic feature that we extract from openSMILE has major 4 features \{i.e. fundamental frequency (f0), voicing, HNR, Loudness\}. This shows the weightage given by the model to predict a particular emotion. To have taken the absolute attention weight for better representation. Here we can observe that while prediction anger emotion and excitement(which has high arousal value) more weightage is given to \textbf{LOUDNESS}(with +ve attention weight) and while prediction sad emotion(which has low arousal value) more weightage is given to \textbf{LOUDNESS}(with -ve attention weight). Similarly for Neutral it is not giving mush weight to the whole prosodic spectrum. On the other had Happy and Frustration has moderate arousal values and same can be observed in the figure.  }
    \includegraphics[totalheight=3.3cm]{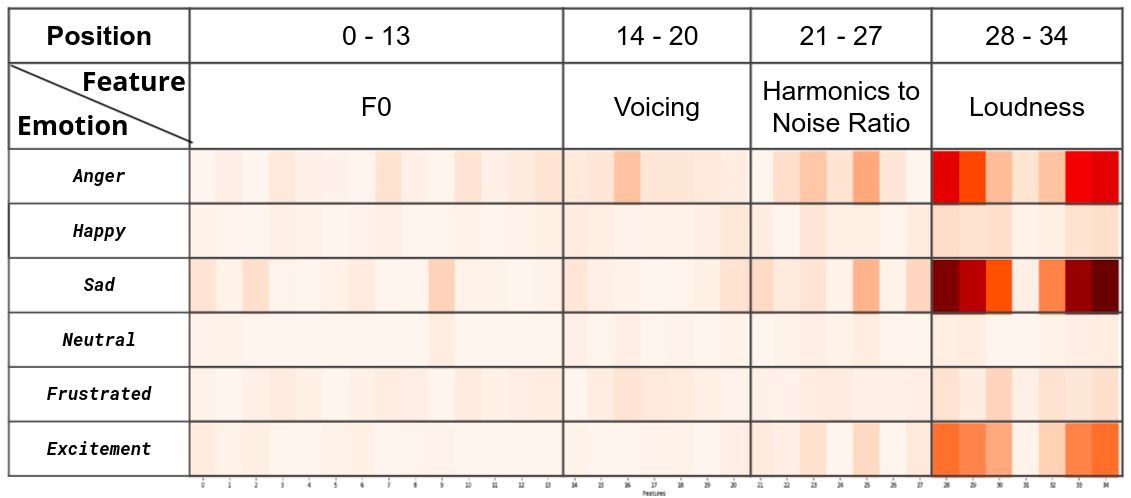}
    \caption{Prosodic feature that we extract from openSMILE has major 4 features \{i.e. fundamental frequency (f0), voicing, HNR, Loudness\}. This shows the weightage given by the model to predict a particular emotion. To have taken the absolute attention weight for better representation. Here we can observe that while predicting anger and excitement(which has high arousal value) more weightage is given to \textbf{LOUDNESS}(with +ve attention weight) and while predicting sad (which has low arousal value) more weightage is given to \textbf{LOUDNESS}(with -ve attention weight). Similarly for Neutral it is not giving much weight to the whole prosodic spectrum. On the other hand, Happy and Frustration have moderate arousal values and same can be observed in the figure.  }
    \label{fig:prosodic}
\end{figure}

%%%%%%%%%%% Character-Label Ratio %%%%%%%%%%%

% Figure \ref{fig:clr} shows the Implicit emotion distribution in every character's sarcastic utterances across the various shows considered in our dataset

\begin{figure*}[!ht]
\centering
\includegraphics[width=.3\textwidth]{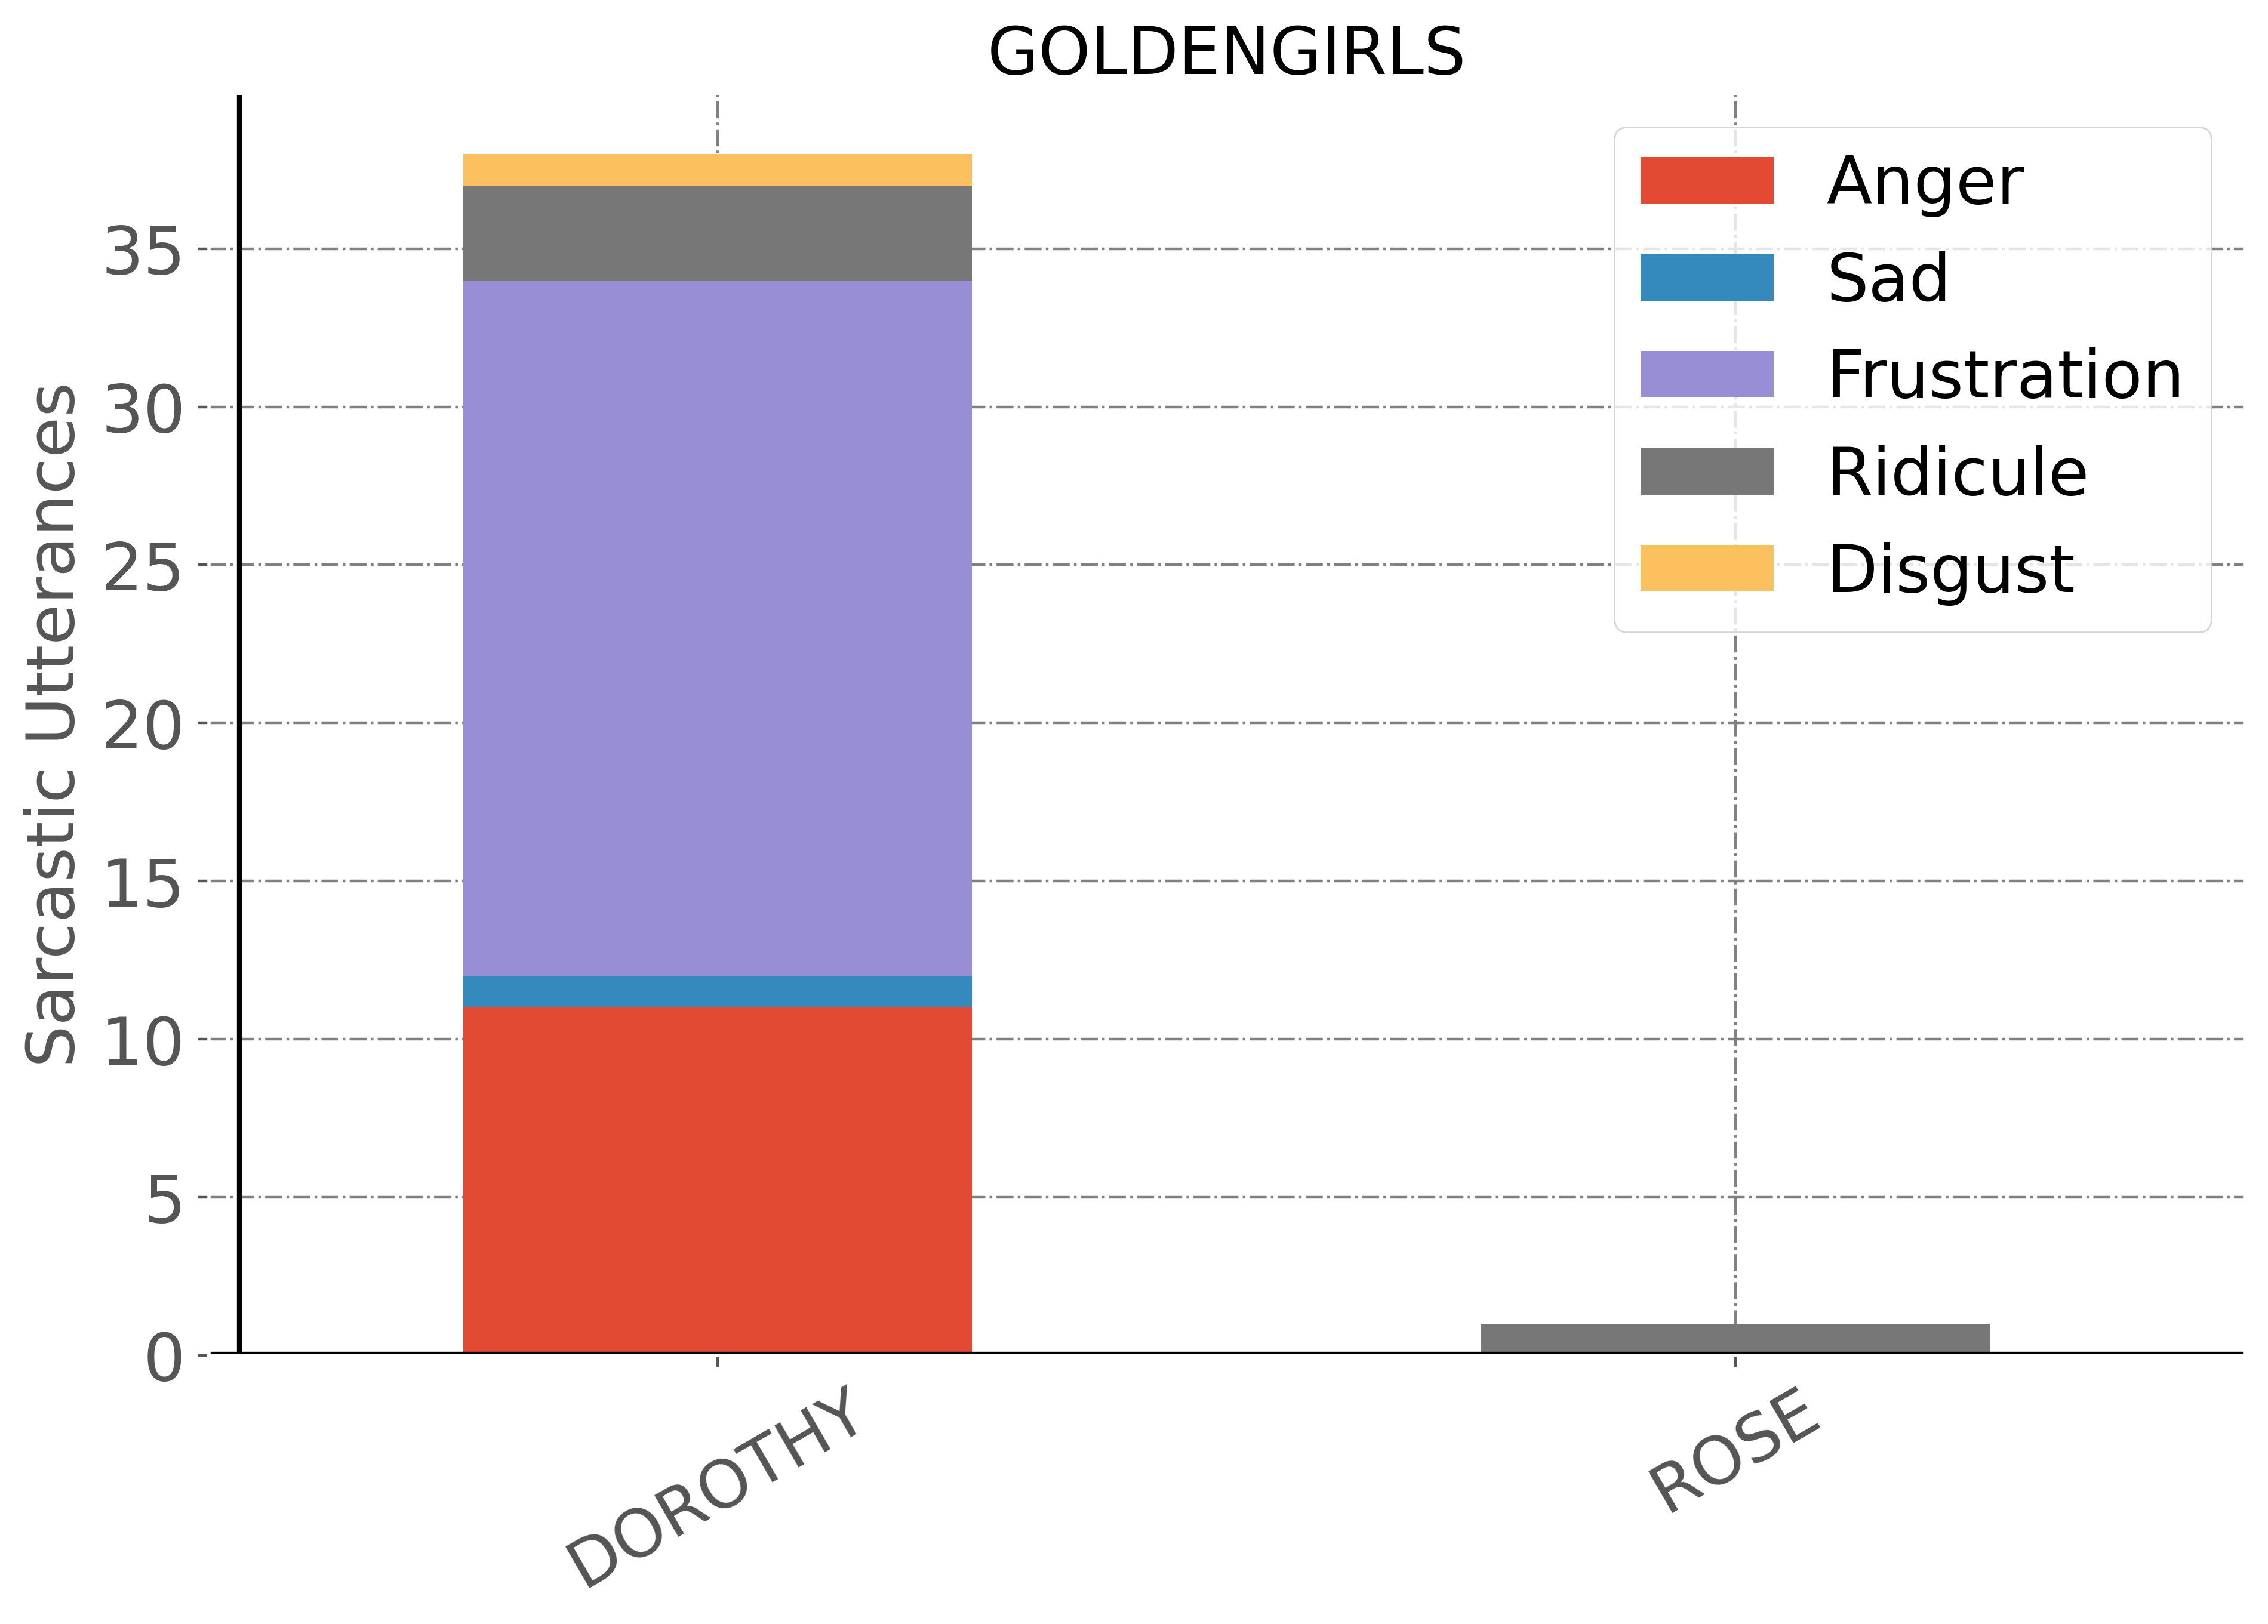}\quad
\includegraphics[width=.3\textwidth]{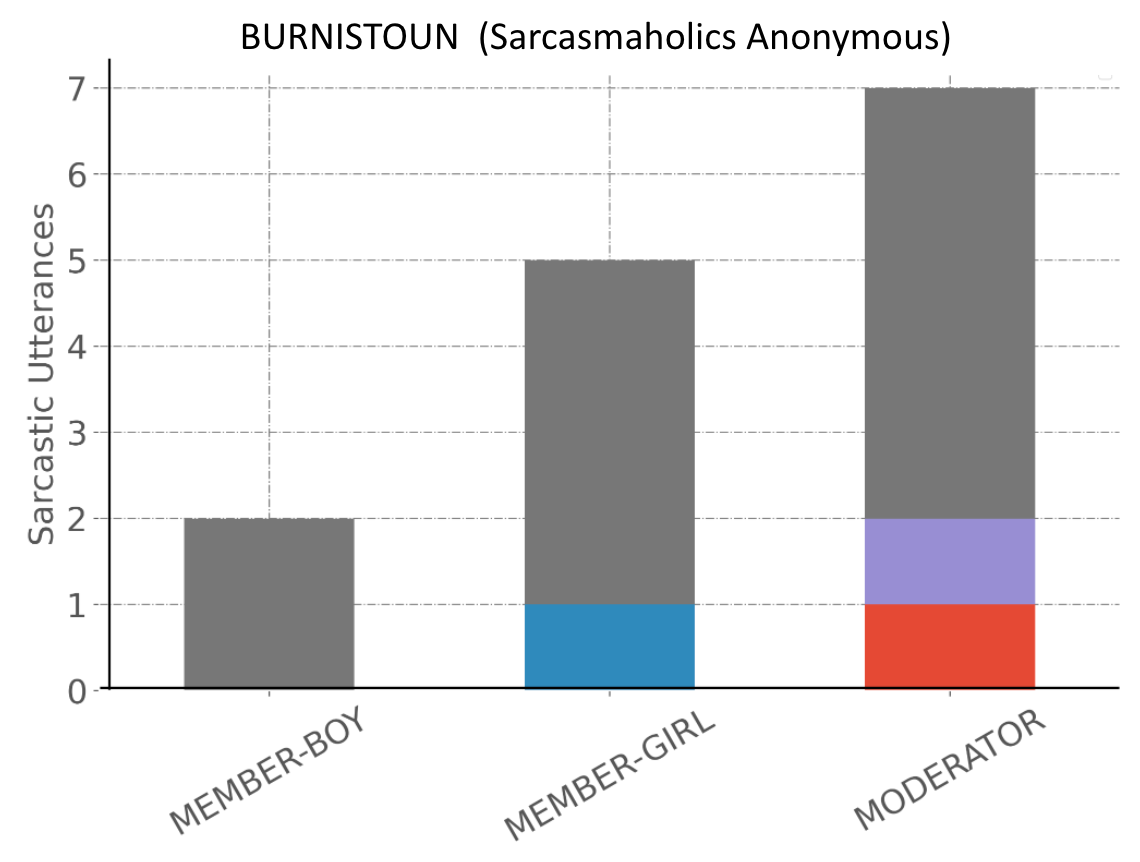}\quad
\includegraphics[width=.3\textwidth]{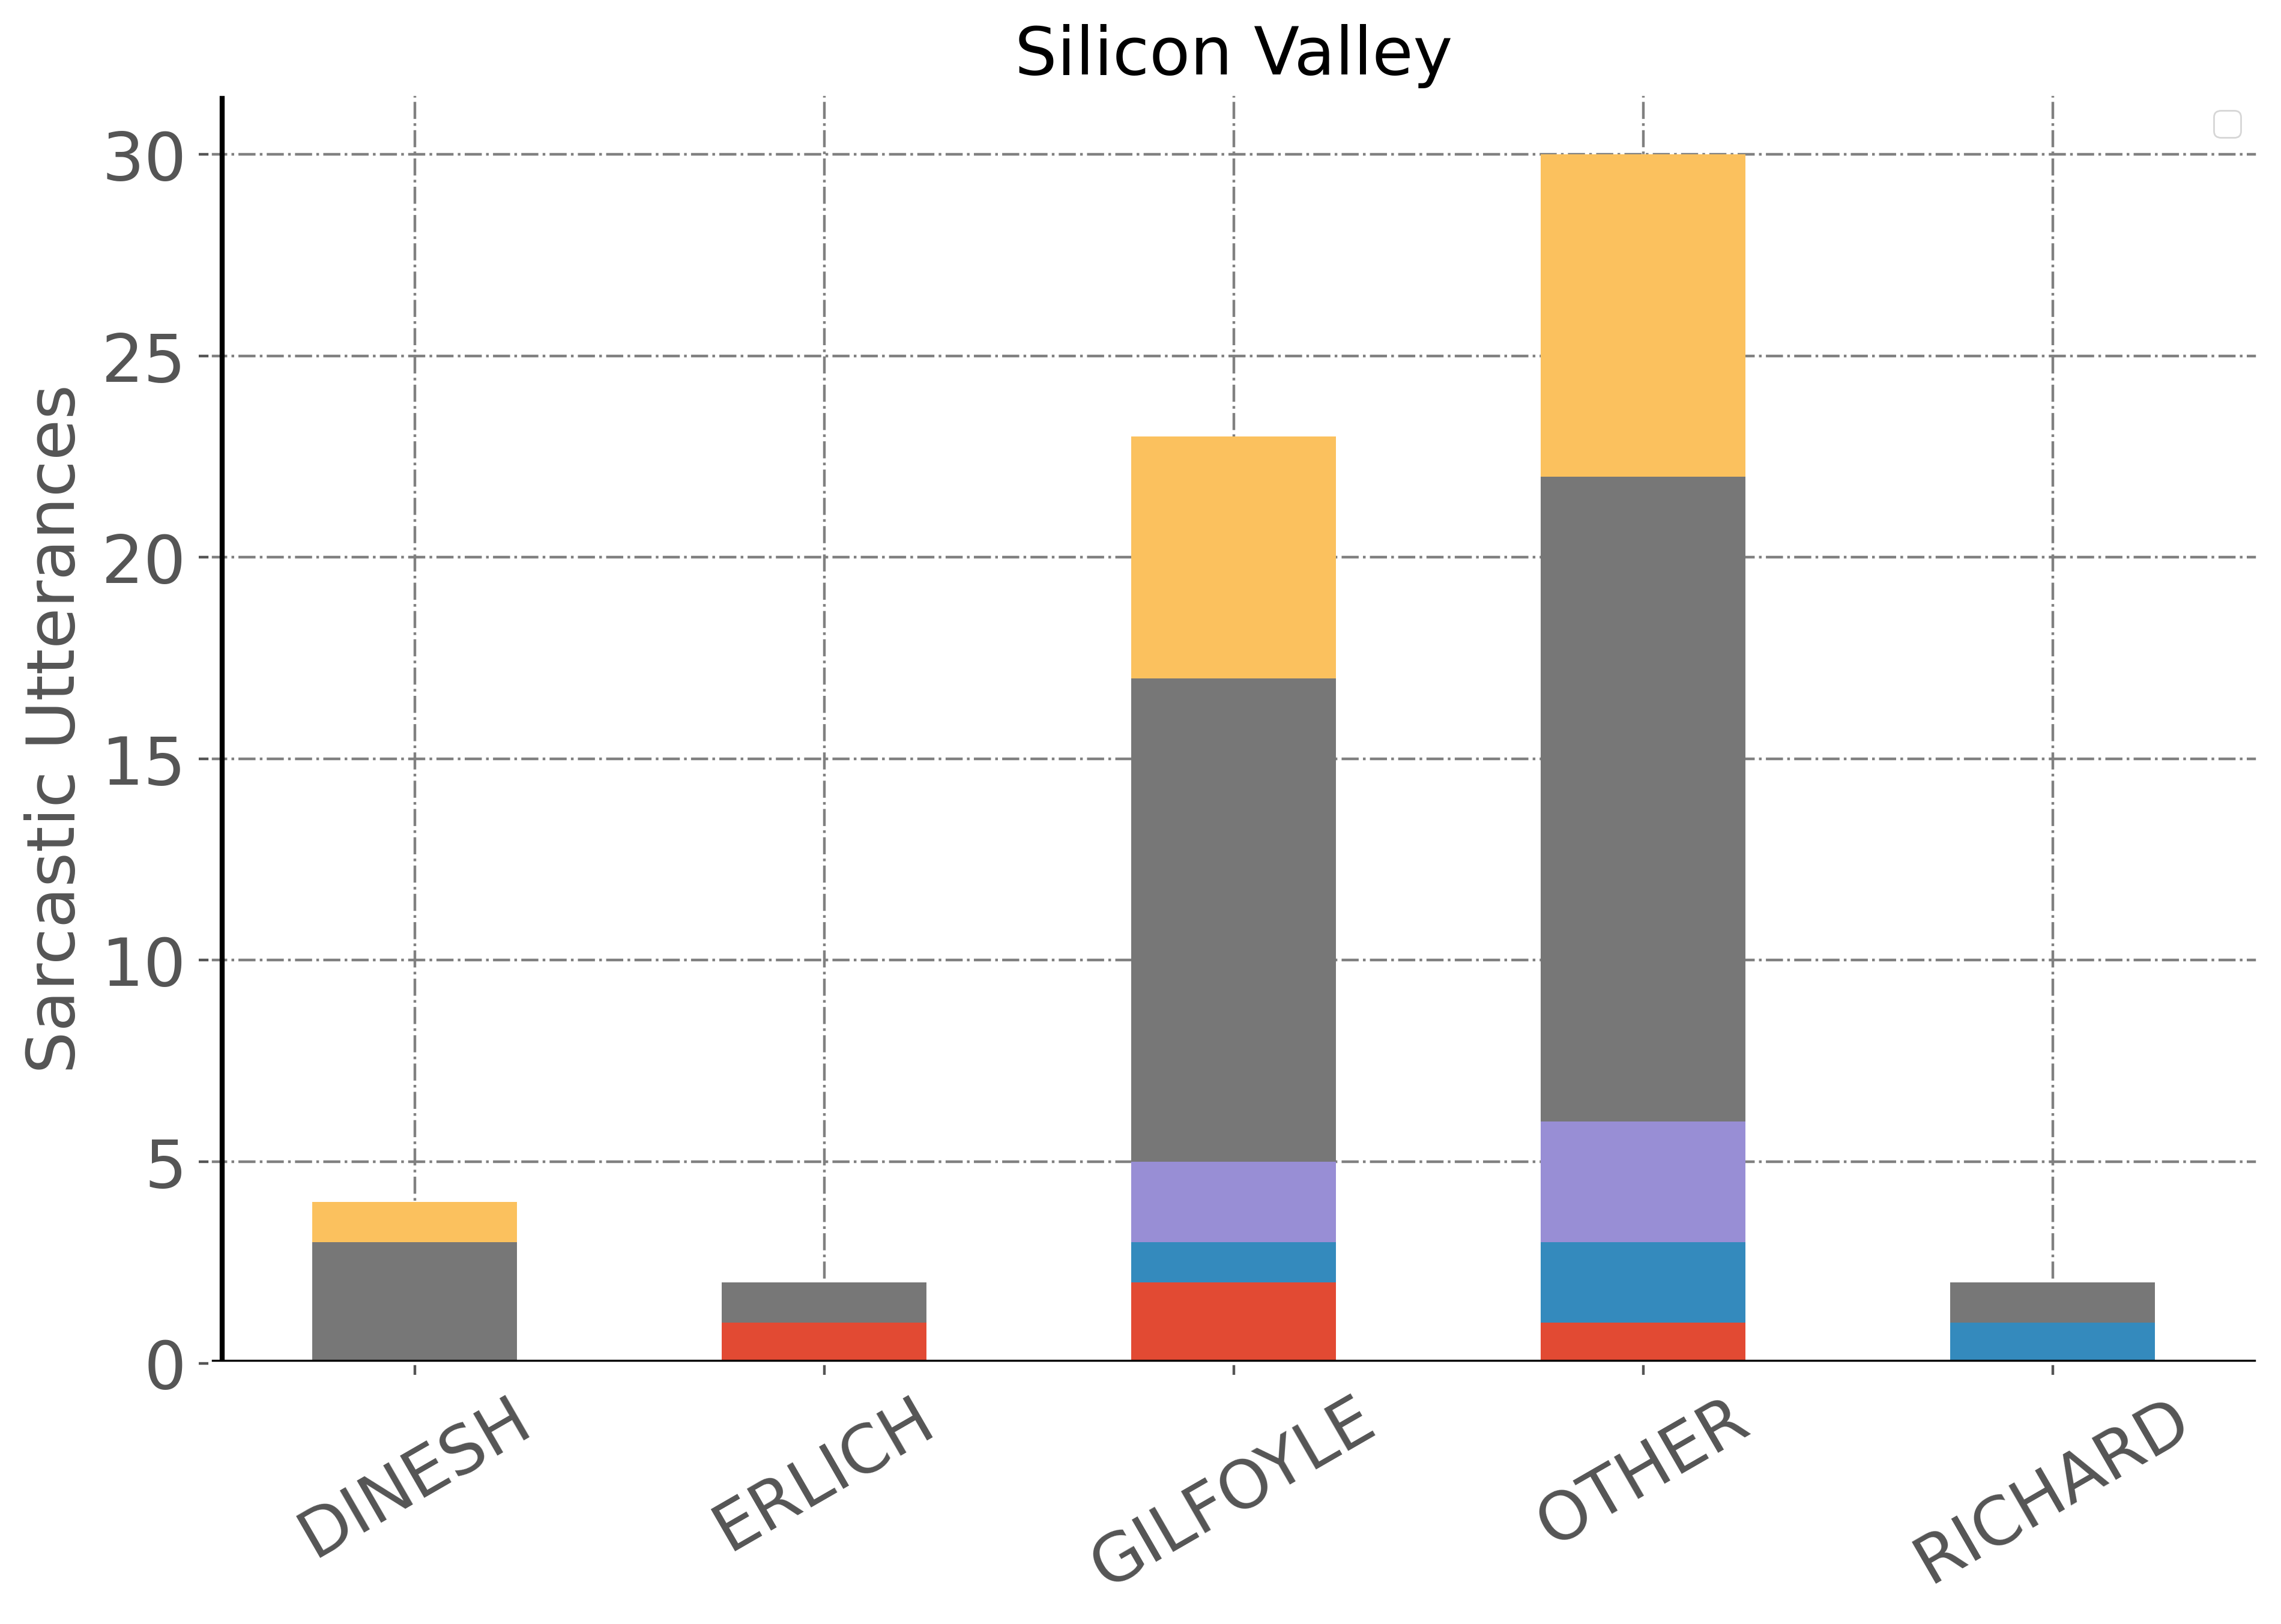}

\medskip

\includegraphics[width=.3\textwidth]{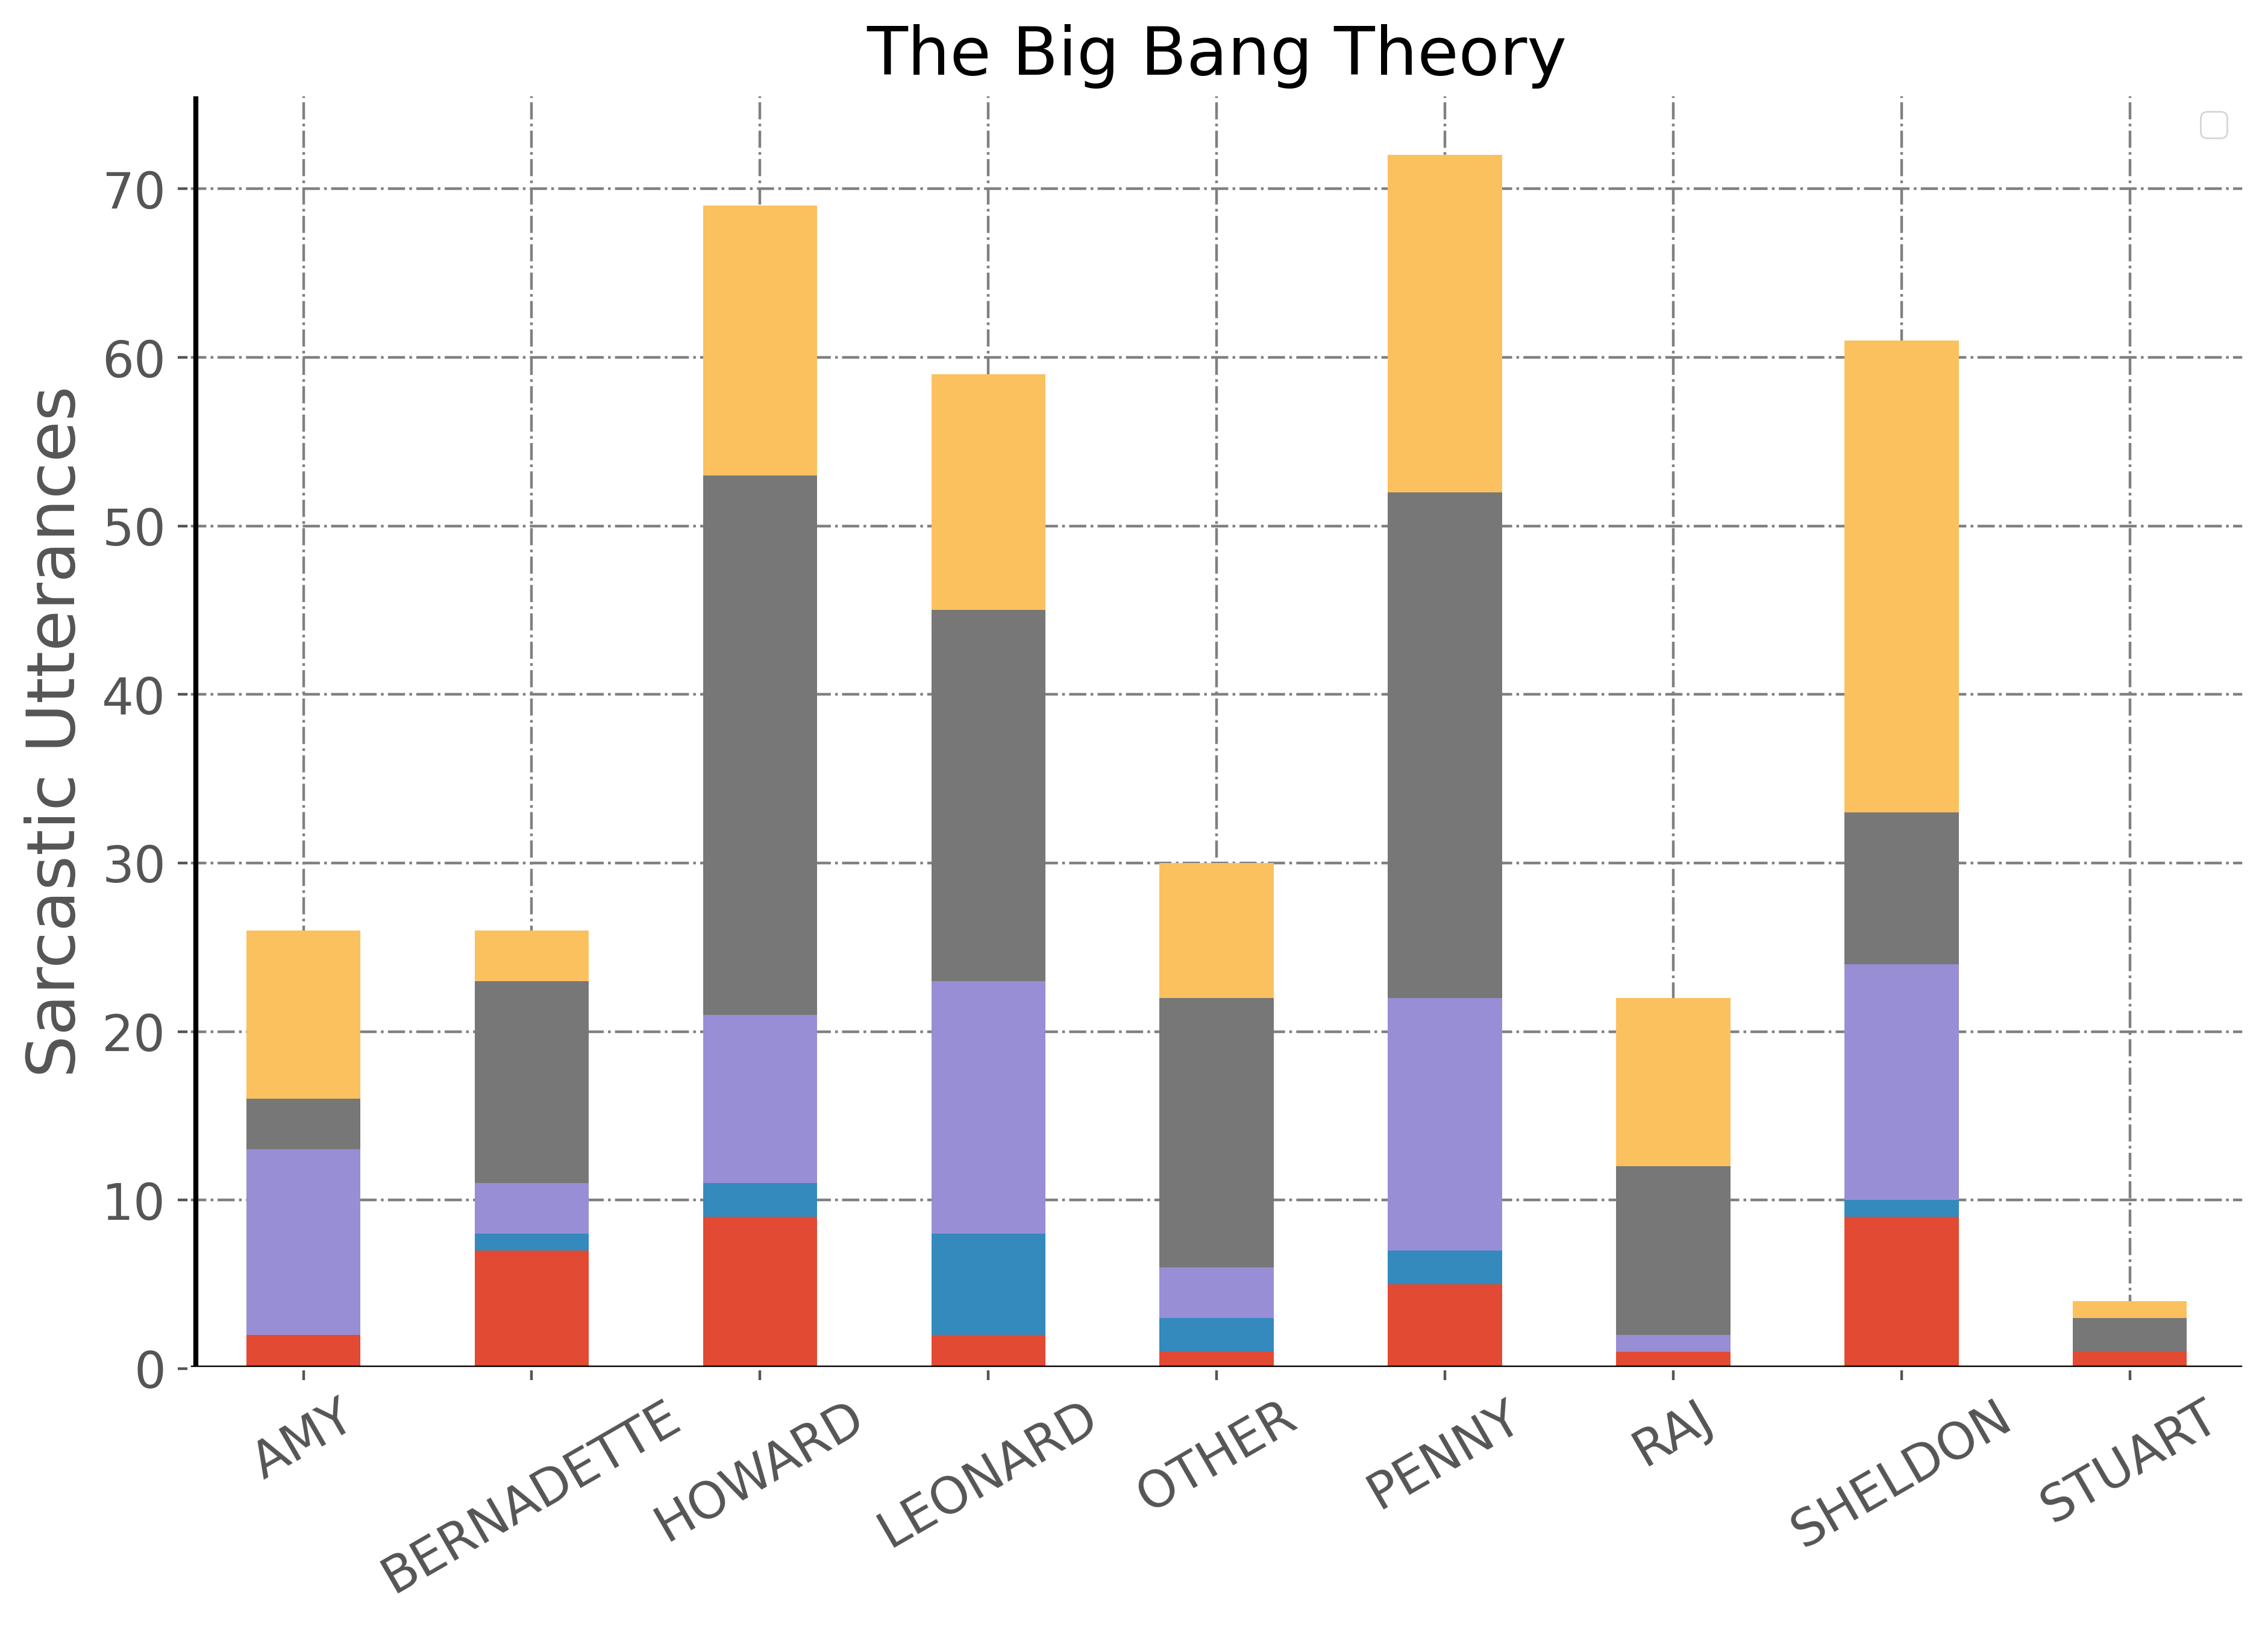}\quad
\includegraphics[width=.3\textwidth]{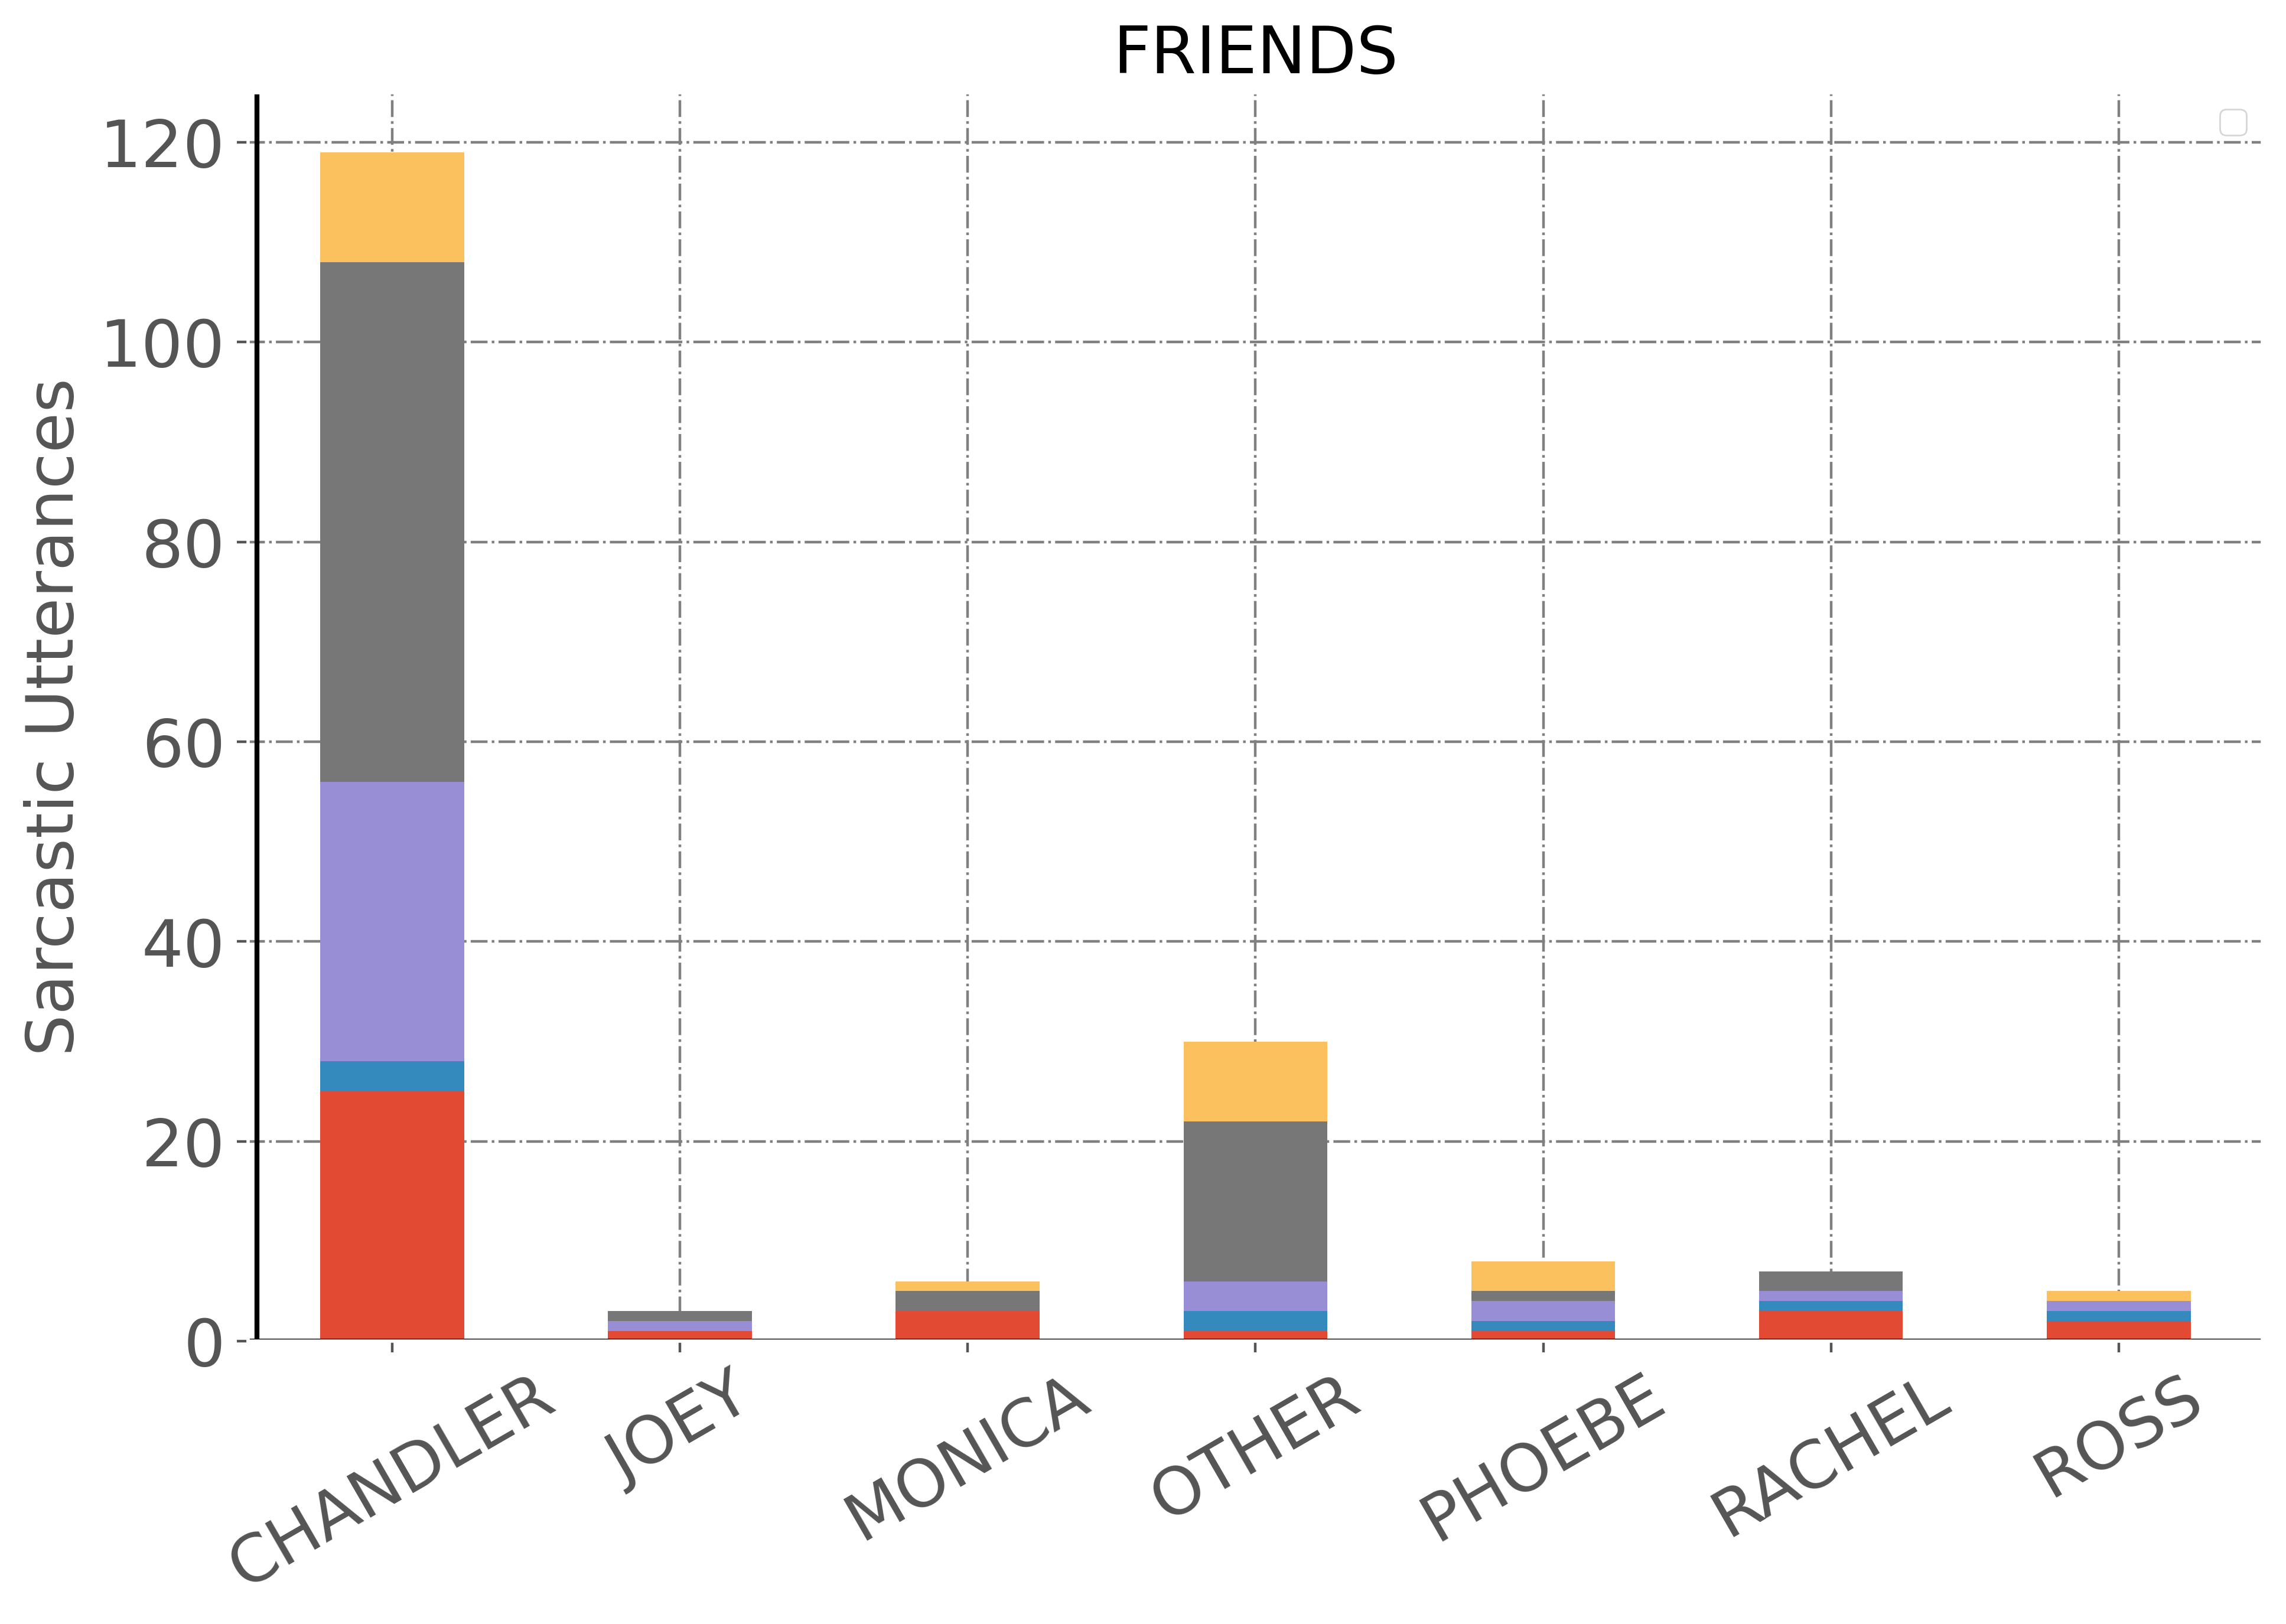}

\caption{Character-label ratio per source  over Implicit Emotion in sarcastic utterances  on MUStARD++ data}
\label{fig:clr}
\end{figure*}

% #############################################################################################################

\section{Additional Results}
\label{sec:additional_results}
The best numbers are reported in the main paper. Table \ref{tab:Sarcasm detection results for MUStARD} shows detailed weighted average results of all modality combinations on the MUStARD data . Similarly Table \ref{tab:Sarcasm detection results for MUStARD++}  shows detailed weighted average results of all modality combinations on the MUStARD++ data. \\
In earlier sections we have presented the detailed weighted average results of all modality combinations for Multiclass experiments for emotion classification. Table \ref{tab:Implicit-Emotion distribution in Sarcastic Utterances-ONEvsREST} and Table \ref{tab:explicit-Emotion distribution in Sarcastic Utterances-ONEvsREST} represent results for ONEvsREST classification experiments of Implicit and Explicit emotion respectively, for different settings.\\
\begin{table*}[ht!]
\centering
\resizebox{\textwidth}{!}{%
\begin{tabular}{c|ccc|ccc|l|ccc|ccc|}
\cline{2-14}
\multicolumn{1}{l|}{}                & \multicolumn{6}{c|}{\textbf{Speaker Independent}}                                             &  & \multicolumn{6}{c|}{\textbf{Speaker Dependent}}                                               \\ \cline{2-7} \cline{9-14} 
\multicolumn{1}{l|}{}                & \multicolumn{3}{c|}{\textbf{w/o Context}}     & \multicolumn{3}{c|}{\textbf{w Context}}       &  & \multicolumn{3}{c|}{\textbf{w/o Context}}     & \multicolumn{3}{c|}{\textbf{w Context}}       \\ \cline{2-7} \cline{9-14} 
\multicolumn{1}{l|}{}                & \textbf{P}    & \textbf{R}    & \textbf{F1}   & \textbf{P}    & \textbf{R}    & \textbf{F1}   &  & \textbf{P}    & \textbf{R}    & \textbf{F1}   & \textbf{P}    & \textbf{R}    & \textbf{F1}   \\ \cline{1-7} \cline{9-14} 
\multicolumn{1}{|c|}{\textbf{T}}     & 65.4          & 65.4          & 65.4          & 67.1          & 67.1          & 67.1          &  & 70.1          & 70.1          & 70.1          & 72.0          & 72.0          & 72.0          \\
\multicolumn{1}{|c|}{\textbf{A}}     & 67.3          & 67.2          & 67.2          & 66.2          & 66.2          & 66.2          &  & 71.2          & 71.2          & 71.2          & 72.2          & 72.2          & 72.2          \\
\multicolumn{1}{|c|}{\textbf{V}}     & 60.9          & 60.9          & 60.9          & 60.9          & 60.9          & 60.8          &  & 69.9          & 69.9          & 69.9          & 72.5          & 72.5          & 72.5          \\
\multicolumn{1}{|c|}{\textbf{T+A}}   & \textbf{68.8} & \textbf{68.8} & \textbf{68.8} & \textbf{68.3} & \textbf{68.3} & \textbf{68.3} &  & 71.9          & 71.9          & 71.9          & 71.9          & 71.9          & 71.9          \\
\multicolumn{1}{|c|}{\textbf{A+V}}   & 65.8          & 65.8          & 65.8          & 65.3          & 65.2          & 65.2          &  & 71.2          & 71.2          & 71.2          & 72.2          & 60.9          & 72.0          \\
\multicolumn{1}{|c|}{\textbf{V+T}}   & 66.5          & 66.5          & 66.5          & 65.9          & 65.9          & 65.9          &  & \textbf{72.8} & \textbf{72.8} & \textbf{72.8} & 71.9          & 71.9          & 71.9          \\
\multicolumn{1}{|c|}{\textbf{T+A+V}} & 68.1          & 68.1          & 68.1          & 67.1          & 67.1          & 67.1          &  & 71.3          & 71.3          & 71.3          & \textbf{72.6} & \textbf{72.6} & \textbf{72.6} \\ \cline{1-7} \cline{9-14} 
% \multicolumn{1}{|l|}{\textbf{$\Delta_{multi - unimodel}$}}            & {\color[HTML]{036400} $\uparrow$ 1.5} & {\color[HTML]{036400} $\uparrow$ 1.5} & {\color[HTML]{036400} $\uparrow$ 1.5}        & {\color[HTML]{036400} $\uparrow$ 1.2} & {\color[HTML]{036400} $\uparrow$ 1.2} & {\color[HTML]{036400} $\uparrow$ 1.2} &  & {\color[HTML]{036400} $\uparrow$ 1.6} & {\color[HTML]{036400} $\uparrow$ 1.6} & {\color[HTML]{036400} $\uparrow$ 1.6} & {\color[HTML]{036400} $\uparrow$ 0.1}          & {\color[HTML]{036400} $\uparrow$ 0.1}          & {\color[HTML]{036400} $\uparrow$ 0.1}          \\
\multicolumn{1}{|l|}{Percentage$\Delta$}           & {\color[HTML]{036400} $\uparrow$ 2.2\%} & {\color[HTML]{036400} $\uparrow$ 2.2\%} & {\color[HTML]{036400} $\uparrow$ 2.2\%}        & {\color[HTML]{036400} $\uparrow$ 1.7\%} & {\color[HTML]{036400} $\uparrow$ 1.7\%} & {\color[HTML]{036400} $\uparrow$ 1.7\%} &  & {\color[HTML]{036400} $\uparrow$ 2.2\%}          & {\color[HTML]{036400} $\uparrow$ 2.2\%}          & {\color[HTML]{036400} $\uparrow$ 2.2\%}          & {\color[HTML]{036400} $\uparrow$ 0.1\%} & {\color[HTML]{036400} $\uparrow$ 0.1\%} & {\color[HTML]{036400} $\uparrow$ 0.1\%} \\ \hline
\end{tabular}%
}
%\captionsetup{justification=centering}
\caption{Sarcasm detection results for MUStARD, Weighted Average}
\label{tab:Sarcasm detection results for MUStARD}
\end{table*}

% ########################################################################%

%#########################################################################################################

\begin{table*}[htp!]
\centering
\resizebox{\textwidth}{!}{%
\begin{tabular}{c|ccc|ccc|l|ccc|ccc|}
\cline{2-14}
\multicolumn{1}{l|}{}                & \multicolumn{6}{c|}{\textbf{Speaker Independent}}                                             &  & \multicolumn{6}{c|}{\textbf{Speaker Dependent}}                                               \\ \cline{2-7} \cline{9-14} 
\multicolumn{1}{l|}{}                & \multicolumn{3}{c|}{\textbf{w/o Context}}     & \multicolumn{3}{c|}{\textbf{w Context}}       &  & \multicolumn{3}{c|}{\textbf{w/o Context}}     & \multicolumn{3}{c|}{\textbf{w Context}}       \\ \cline{2-7} \cline{9-14} 
\multicolumn{1}{l|}{}                & \textbf{P}    & \textbf{R}    & \textbf{F1}   & \textbf{P}    & \textbf{R}    & \textbf{F1}   &  & \textbf{P}    & \textbf{R}    & \textbf{F1}   & \textbf{P}    & \textbf{R}    & \textbf{F1}   \\ \cline{1-7} \cline{9-14} 
\multicolumn{1}{|c|}{\textbf{T}}     & 67.9 & 67.7 & 67.7 & 69.3 & 69.2 & 69.2 && 69.4 & 69.3 & 69.3 & 70.2 & 70 & 70          \\
\multicolumn{1}{|c|}{\textbf{A}}     & 63.4          & 63.4          & 63.4          & 64.9          & 64.9          & 64.9          &  & 64.6          & 64.6          & 64.6          & 64.5          & 64.5          & 64.5          \\
\multicolumn{1}{|c|}{\textbf{V}}     & 60         &60         & 60         & 60 &60 &60          &  & 62          & 62          & 62          & 63          &63          & 63        \\
\multicolumn{1}{|c|}{\textbf{T+A}}   & 68.8 & 68.6 & 68.7 &70.2 & 70.2 & 70.2 && 69.8 & 69.5 & 69.5 & 69.2 & 69.1 & 69.1                  \\
\multicolumn{1}{|c|}{\textbf{A+V}}   & 63& 63& 63 &64 &64 &64 &&65 &65 &65  &65 &65 &65          \\
\multicolumn{1}{|c|}{\textbf{V+T}}   & 68 & 68 & 68 & 68 & 68 & 68 && 68 & 68 & 68 & 69 & 69 & 69         \\
\multicolumn{1}{|c|}{\textbf{T+A+V}} &70 & 70 & 70 & 69 & 69 & 69 && 71 & 71 & 71 & 69 & 69 & 69  \\ \cline{1-7} \cline{9-14} 
% \multicolumn{1}{|l|}{\textbf{$\Delta_{multi - unimodel}$}}            & {\color[HTML]{036400} $\uparrow$ 2.2} & {\color[HTML]{036400} $\uparrow$ 2.2} & {\color[HTML]{036400} $\uparrow$ 2.2}        & {\color[HTML]{036400} $\uparrow$ 3.2} & {\color[HTML]{036400} $\uparrow$ 3.2} & {\color[HTML]{036400} $\uparrow$ 3.2} &  & {\color[HTML]{036400} $\uparrow$ 2.1} & {\color[HTML]{036400} $\uparrow$ 2.2} & {\color[HTML]{036400} $\uparrow$ 2.2} & {\color[HTML]{036400} $\uparrow$ 3.2}          & {\color[HTML]{036400} $\uparrow$ 3.2}          & {\color[HTML]{036400} $\uparrow$ 3.2}          \\
% \multicolumn{1}{|l|}{Percentage$\Delta$}           & {\color[HTML]{036400} $\uparrow$ 3.3\%} & {\color[HTML]{036400} $\uparrow$ 3.3\%} & {\color[HTML]{036400} $\uparrow$ 3.3\%}        & {\color[HTML]{036400} $\uparrow$ 4.8\%} & {\color[HTML]{036400} $\uparrow$ 4.8\%} & {\color[HTML]{036400} $\uparrow$ 4.8\%} & & {\color[HTML]{036400} 3.1\%}& {\color[HTML]{036400} 3.3\%}          & {\color[HTML]{036400} $\uparrow$ 3.3\%}          & {\color[HTML]{036400} $\uparrow$ 4.7\%} & {\color[HTML]{036400} $\uparrow$ 4.7\%} & {\color[HTML]{036400} $\uparrow$ 4.7\%} \\ \hline
\end{tabular}%
}
\captionsetup{justification=centering}
\caption{Sarcasm detection results for \textbf{MUStARD++}, Weighted Average}
\label{tab:Sarcasm detection results for MUStARD++}
\end{table*}

% ###############################################################################################################
\begin{table*}[ht!]
\centering
\resizebox{\textwidth}{!}{%
\begin{tabular}{c|ccc|ccc|l|ccc|ccc|}
\cline{2-14}
\multicolumn{1}{l|}{}                & \multicolumn{6}{c|}{\textbf{Speaker Independent}}                                             &  & \multicolumn{6}{c|}{\textbf{Speaker Dependent}}                                               \\ \cline{2-7} \cline{9-14} 
\multicolumn{1}{l|}{}                & \multicolumn{3}{c|}{\textbf{w/o Context}}     & \multicolumn{3}{c|}{\textbf{w Context}}       &  & \multicolumn{3}{c|}{\textbf{w/o Context}}     & \multicolumn{3}{c|}{\textbf{w Context}}       \\ \cline{2-7} \cline{9-14} 
\multicolumn{1}{l|}{}                & \textbf{P}    & \textbf{R}    & \textbf{F1}   & \textbf{P}    & \textbf{R}    & \textbf{F1}   &  & \textbf{P}    & \textbf{R}    & \textbf{F1}   & \textbf{P}    & \textbf{R}    & \textbf{F1}   \\ \cline{1-7} \cline{9-14} 
\multicolumn{1}{|c|}{\textbf{T}}     & 30.6          & 32.6          & 31.0          & 30.4          & 33.1          & 31.2          &  & 30.8          & 32.9          & 31.4          & 31.0          & 35.1          & 33.8          \\
\multicolumn{1}{|c|}{\textbf{A}}     & 29.4          & 30.3          & 29.7          & 295          & 30.4          & 29.9          &  & 30.7          & 31.1          & 30.6          & 29.4          & 30.6          & 29.7          \\
\multicolumn{1}{|c|}{\textbf{V}}     & 31.7          & 34.6          & 32.9          & 32.7          & 31.3         & 31.8          &  & 32.2          & 33.6          & 32.5          & 31.1          & 32.8          & 31.8          \\
\multicolumn{1}{|c|}{\textbf{T+A}}   & 32.4          & 34.4          & 32.8          & \textbf{33.5} & \textbf{36.6} & \textbf{34.5} &  & 32.0          & 31.6          & 31.5          & 32.1          & 35.1          & 32.9          \\
\multicolumn{1}{|c|}{\textbf{A+V}}   & 29.8          & 31.6          & 30.5          & 29.3          & 33.4          & 30.6          &  & 31.8          & 33.4          & 32.5          & 30.2          & 32.6          & 306          \\
\multicolumn{1}{|c|}{\textbf{V+T}}   & \textbf{32.2} & \textbf{35.8} & \textbf{33.0} & 32.2          & 33.3          & 32.7          &  & 33.2          & 34.8          & 33.5          & 33.1          & 33.8          & 33.3          \\
\multicolumn{1}{|c|}{\textbf{T+A+V}} & 31.8          & 35.3          & 31.7          & 32.4          & 36.4          & 32.5          &  & \textbf{31.9} & \textbf{32.6} & \textbf{32.1} & \textbf{35.2} & \textbf{36.4} & \textbf{35.6} \\  \cline{1-7} \cline{9-14} 
% \multicolumn{1}{|l|}{\textbf{$\Delta_{multi - unimodel}$}}            & {\color[HTML]{036400} $\uparrow$ 0.5} & {\color[HTML]{036400} $\uparrow$ 1.2} & {\color[HTML]{036400} $\uparrow$ 0.1}        & {\color[HTML]{036400} $\uparrow$ 0.8} & {\color[HTML]{036400} $\uparrow$ 3.5} & {\color[HTML]{036400} $\uparrow$ 2.7} &  & {\color[HTML]{036400} $\uparrow$ 1.0} & {\color[HTML]{036400} $\uparrow$ 1.2} & {\color[HTML]{036400} $\uparrow$ 1.0} & {\color[HTML]{036400} $\uparrow$ 4.1}          & {\color[HTML]{036400} $\uparrow$ 1.3}          & {\color[HTML]{036400} $\uparrow$ 1.8}          \\
\multicolumn{1}{|l|}{Percentage$\Delta$}           & {\color[HTML]{036400} $\uparrow$ 1.5\%} & {\color[HTML]{036400} $\uparrow$ 3.4\%} & {\color[HTML]{036400} $\uparrow$ 0.3\%}        & {\color[HTML]{036400} $\uparrow$ 2.4\%} & {\color[HTML]{036400} $\uparrow$ 10.5\%} & {\color[HTML]{036400} $\uparrow$ 8.5\%} &  & {\color[HTML]{036400} $\uparrow$ 3.1\%}          & {\color[HTML]{036400} $\uparrow$ 3.6\%}          & {\color[HTML]{036400} $\uparrow$ 3.1\%}          & {\color[HTML]{036400} $\uparrow$ 13.2\%} & {\color[HTML]{036400} $\uparrow$ 3.7\%} & {\color[HTML]{036400} $\uparrow$ 5.3\%} \\ \hline
\end{tabular}%
}
\captionsetup{justification=centering}
\caption{Implicit Emotion Classification in Sarcastic Utterance(ONEvsREST) Weighted Average}
\label{tab:Implicit-Emotion distribution in Sarcastic Utterances-ONEvsREST}
\end{table*}

%#################################################################################################

\begin{table*}[ht!]
\centering
\resizebox{\textwidth}{!}{%
\begin{tabular}{c|ccc|ccc|l|ccc|ccc|}
\cline{2-14}
\multicolumn{1}{l|}{}                & \multicolumn{6}{c|}{\textbf{Speaker Independent}}                                             &  & \multicolumn{6}{c|}{\textbf{Speaker Dependent}}                                               \\ \cline{2-7} \cline{9-14} 
\multicolumn{1}{l|}{}                & \multicolumn{3}{c|}{\textbf{w/o Context}}     & \multicolumn{3}{c|}{\textbf{w Context}}       &  & \multicolumn{3}{c|}{\textbf{w/o Context}}     & \multicolumn{3}{c|}{\textbf{w Context}}       \\ \cline{2-7} \cline{9-14} 
\multicolumn{1}{l|}{}                & \textbf{P}    & \textbf{R}    & \textbf{F1}   & \textbf{P}    & \textbf{R}    & \textbf{F1}   &  & \textbf{P}    & \textbf{R}    & \textbf{F1}   & \textbf{P}    & \textbf{R}    & \textbf{F1}   \\ \cline{1-7} \cline{9-14} 
\multicolumn{1}{|c|}{\textbf{T}}     & 31.5          & 30.8          & 31.1          & 34.0          & 37.8          & 35.3          &  & 32.6          & 34.1          & 33.1          & 33.3          & 36.1          & 34.3          \\
\multicolumn{1}{|c|}{\textbf{A}}     & 28.3          & 31.8          & 29.3          & 27.7          & 30.8          & 28 8         &  & 29.8          & 33.4          & 31.3          & 30.5          & 35.9          & 31.6          \\
\multicolumn{1}{|c|}{\textbf{V}}     & 26.6          & 30.6          & 28.2          & 28.3          & 30.1    & 29.0          &  & 29.3          & 33.6          & 30.9          & 29.0          & 33.4          & 30.6          \\
\multicolumn{1}{|c|}{\textbf{T+A}}   & \textbf{38.4 }         & \textbf{39.8}          & \textbf{39.0}          & 40.1          & 41.6          & 40.6          &  & {34.9} & {36.9} & {35.8} & \textbf{37.3}          & \textbf{38.8}          & \textbf{37.9}          \\
\multicolumn{1}{|c|}{\textbf{A+V}}   & 29.6          & 31.9          & 30.4          & 27.7          & 30.0          & 28.6          &  & 30.1          & 34.3          & 31.2          & 29.8          & 31.9          & 30.7          \\
\multicolumn{1}{|c|}{{V+T}}   & {37.7} & {40.6} & {38.8} & \textbf{42.0} & \textbf{44.2} & \textbf{42.6} &  & \textbf{36.3}          &\textbf{ 38.4}          & \textbf{37.2}          & {37.0} & {38.8} & {37.7} \\
\multicolumn{1}{|c|}{\textbf{T+A+V}} & 35.2          & 39.6          & 36.4          & 36.1          & 39.4          & 37.3          &   & 35.2          & 38.4          & 36.4          & 33.8          & 36.1          & 34.8          \\ \cline{1-7} \cline{9-14} 
% \multicolumn{1}{|l|}{\textbf{$\Delta_{multi - unimodel}$}}            & {\color[HTML]{036400} $\uparrow$ 6.9} & {\color[HTML]{036400} $\uparrow$ 8.0} & {\color[HTML]{036400} $\uparrow$ 7.9}        & {\color[HTML]{036400} $\uparrow$ 8.0} & {\color[HTML]{036400} $\uparrow$ 6.5} & {\color[HTML]{036400} $\uparrow$ 7.5} &  & {\color[HTML]{036400} $\uparrow$ 3.7} & {\color[HTML]{036400} $\uparrow$ 4.3} & {\color[HTML]{036400} $\uparrow$ 4.1} & {\color[HTML]{036400} $\uparrow$ 4.0}          & {\color[HTML]{036400} $\uparrow$ 2.7}          & {\color[HTML]{036400} $\uparrow$ 3.6}          \\
\multicolumn{1}{|l|}{Percentage$\Delta$}           & {\color[HTML]{036400} $\uparrow$ 21.9\%} & {\color[HTML]{036400} $\uparrow$ 25.1\%} & {\color[HTML]{036400} $\uparrow$ 25.4\%}        & {\color[HTML]{036400} $\uparrow$ 23.5\%} & {\color[HTML]{036400} $\uparrow$ 17.1\%} & {\color[HTML]{036400} $\uparrow$ 21.2\%} &  & {\color[HTML]{036400} $\uparrow$ 11.3\%}          & {\color[HTML]{036400} $\uparrow$ 12.6\%}          & {\color[HTML]{036400} $\uparrow$ 12.9\%}          & {\color[HTML]{036400} $\uparrow$ 12.0\%} & {\color[HTML]{036400} $\uparrow$ 7.5\%} & {\color[HTML]{036400} $\uparrow$ 10.5\%} \\ \hline
\end{tabular}%
}
\captionsetup{justification=centering}
\caption{Explicit Emotion Classification in Sarcastic Utterance(ONEvsREST) Weighted Average}
\label{tab:explicit-Emotion distribution in Sarcastic Utterances-ONEvsREST}
\end{table*}

%#################################################################################################
%%%%% Apoorva's Results
\begin{table*}[h!]
% \small
\centering
% \resizebox{\textwidth}{!}
{%
\begin{tabular}{|c|ccc|ccc|}

\cline{2-7}
\multicolumn{1}{l|}{}                & \multicolumn{6}{c|}{\textbf{Speaker Independent}}                                                                              \\ \cline{2-7} 
\multicolumn{1}{l|}{}                & \multicolumn{3}{c|}{\textbf{w/o Context}}     & \multicolumn{3}{c|}{\textbf{w Context}} \\ \cline{2-7}  
\multicolumn{1}{l|}{}                & \textbf{P}    & \textbf{R}    & \textbf{F1}   & \textbf{P}    & \textbf{R}    & \textbf{F1}    \\ \cline{1-7} 
\multicolumn{1}{|c|}{\textbf{T}}     & 31.86$\pm$0.9          & 32.45$\pm$0.81          & \textcolor{red}{32.13$\pm$0.85}        & 30.75$\pm$0.74          & 31.15$\pm$0.64         & 30.93$\pm$0.7          \\
\multicolumn{1}{|c|}{\textbf{A}}     & 24.82$\pm$1.75          & 25.16$\pm$1.6          & 24.96$\pm$1.68          & 25.19$\pm$1.32          & 25.12$\pm$1.55          & 25.14$\pm$1.44           \\
\multicolumn{1}{|c|}{\textbf{V}}     & 29.53$\pm$1.05          & 29.98$\pm$1.03          & 29.7$\pm$1.03          & 29.94$\pm$1.49          & 30.72$\pm$2.69          & 30.17$\pm$2.09               \\
\multicolumn{1}{|c|}{\textbf{T+A}}   & 31.72$\pm$0.62          & 31.71$\pm$0.49         & 31.7$\pm$0.55          & 33.06$\pm$1.08         & 33.58$\pm$1.05          & \textcolor{red}{33.29$\pm$1.05}             \\
\multicolumn{1}{|c|}{\textbf{A+V}}   & 25.86$\pm$1.78          & 26.42$\pm$1.89          & 26.11$\pm$1.83         & 25.42$\pm$0.98          & 25.79$\pm$1.16          & 25.6$\pm$1.06         \\
\multicolumn{1}{|c|}{\textbf{V+T}}   & 31.8$\pm$0.83    & 32.15$\pm$0.82 & 31.96$\pm$0.83  & 31.83$\pm$1.3  & 32.11$\pm$1.9  & 31.94$\pm$1.23 \\
\multicolumn{1}{|c|}{\textbf{T+A+V}} & 31.22$\pm$0.75         & 31.65$\pm$0.97         & 31.42$\pm$0.85         & 30.49$\pm$0.94         & 30.82$\pm$0.95          & 30.63$\pm$0.93           \\\cline{1-7} 
% \multicolumn{1}{|l|}{\textbf{$\Delta_{multi - unimodel}$}}            & {\color[HTML]{036400} $\uparrow$ 4.7} & {\color[HTML]{036400} $\uparrow$ 4.3} & {\color[HTML]{036400} $\uparrow$ 4.7}        & {\color[HTML]{036400} $\uparrow$ 0.6} & {\color[HTML]{036400} $\uparrow$ 1.0} & {\color[HTML]{036400} $\uparrow$ 1.2} &  & {\color[HTML]{036400} $\uparrow$ 0.3} & {\color[HTML]{036400} $\uparrow$ 0.2} & {\color[HTML]{036400} $\uparrow$ 0.2} & {\color[HTML]{036400} $\uparrow$ 3.3}          & {\color[HTML]{036400} $\uparrow$ 3.3}          & {\color[HTML]{036400} $\uparrow$ 2.4}          \\
% \multicolumn{1}{|l|}{\textbf{\%$\Delta$Unimodal}}           & {\color[HTML]{036400} $\uparrow$ 15.3\%} & {\color[HTML]{036400} $\uparrow$ 13.3\%} & {\color[HTML]{036400} $\uparrow$ 15.1\%}        & {\color[HTML]{036400} $\uparrow$ 1.8\%} & {\color[HTML]{036400} $\uparrow$ 2.9\%} & {\color[HTML]{036400} $\uparrow$ 3.6\%} &  & {\color[HTML]{036400} $\uparrow$ 0.9\%}          & {\color[HTML]{036400} $\uparrow$ 0.6\%}          & {\color[HTML]{036400} $\uparrow$ 0.6\%}          & {\color[HTML]{036400} $\uparrow$ 10.7\%} & {\color[HTML]{036400} $\uparrow$ 10.3\%} & {\color[HTML]{036400} $\uparrow$ 7.52\%} \\
\hline
\end{tabular}%
}
\captionsetup{justification=centering}
\caption{Mean, std-dev of 5 runs for Implicit Emotion Classification in Sarcastic Utterance(Multiclass) on MUStARD++ in a speaker independent setting}
\label{tab:implicit-Emotion distribution in Sarcastic Utterances-multiclass-speaker-independent}
\end{table*}

% %%%%% Apoorva's Results
\begin{table*}[h!]
% \small
\centering

% \resizebox{\textwidth}{!}
{%
\begin{tabular}{|c|ccc|ccc|}
\cline{2-7}
\multicolumn{1}{l|}{}                & \multicolumn{6}{c|}{\textbf{Speaker Dependent}}                                               \\ \cline{2-7} 
\multicolumn{1}{l|}{}                & \multicolumn{3}{c|}{\textbf{w/o Context}}     & \multicolumn{3}{c|}{\textbf{w Context}}  \\ \cline{2-7} 
\multicolumn{1}{l|}{}                & \textbf{P}    & \textbf{R}    & \textbf{F1}   & \textbf{P}    & \textbf{R}    & \textbf{F1}  \\ \cline{1-7}  
\multicolumn{1}{|c|}{\textbf{T}} & 31.17$\pm$0.88          & 31.81$\pm$0.94           & 31.45$\pm$0.93         & 30.44$\pm$1.04          & 30.82$\pm$1.28          & 30.58$\pm$1.17          \\
\multicolumn{1}{|c|}{\textbf{A}}     &  27.91$\pm$0.82          & 30.92$\pm$2.38          & 28.76$\pm$1.18          & 27.06$\pm$0.91         & 27.22$\pm$0.7          & 27.11$\pm$0.81          \\
\multicolumn{1}{|c|}{\textbf{V}}      & 33.27$\pm$2.87          & 37.4$\pm$2.84          & \textcolor{red}{33.24$\pm$2.23}          & 30.15$\pm$0.99          & 31.78$\pm$1.76          & 30.15$\pm$1.3         \\
\multicolumn{1}{|c|}{\textbf{T+A}}   &  28.0$\pm$0.99          &29.02$\pm$0.96          & 28.91$\pm$0.94         & 31.11$\pm$0.67          & 31.38$\pm$0.7          & 31.2$\pm$0.68         \\
\multicolumn{1}{|c|}{\textbf{A+V}}   &  25.57$\pm$1.38          & 25.99$\pm$1.89          & 25.75$\pm$1.60         & 25.88$\pm$0.74          & 26.26$\pm$1.30          & 26.03$\pm$0.98          \\
\multicolumn{1}{|c|}{\textbf{V+T}}   & 30.71$\pm$0.63          & 30.95$\pm$0.67         & 30.81$\pm$0.63          & 31.01$\pm$0.62         & 31.31$\pm$0.54         & \textcolor{red}{31.33$\pm$0.56}          \\
\multicolumn{1}{|c|}{\textbf{T+A+V}} &  29.34$\pm$0.83 & 29.28$\pm$0.93 & 29.25$\pm$0.88 & 29.34$\pm$1.03 & 29.18$\pm$0.85 & 29.13$\pm$0.94 \\\cline{1-7}
% \multicolumn{1}{|l|}{\textbf{$\Delta_{multi - unimodel}$}}            & {\color[HTML]{036400} $\uparrow$ 4.7} & {\color[HTML]{036400} $\uparrow$ 4.3} & {\color[HTML]{036400} $\uparrow$ 4.7}        & {\color[HTML]{036400} $\uparrow$ 0.6} & {\color[HTML]{036400} $\uparrow$ 1.0} & {\color[HTML]{036400} $\uparrow$ 1.2} &  & {\color[HTML]{036400} $\uparrow$ 0.3} & {\color[HTML]{036400} $\uparrow$ 0.2} & {\color[HTML]{036400} $\uparrow$ 0.2} & {\color[HTML]{036400} $\uparrow$ 3.3}          & {\color[HTML]{036400} $\uparrow$ 3.3}          & {\color[HTML]{036400} $\uparrow$ 2.4}          \\
% \multicolumn{1}{|l|}{\textbf{\%$\Delta$Unimodal}}           & {\color[HTML]{036400} $\uparrow$ 15.3\%} & {\color[HTML]{036400} $\uparrow$ 13.3\%} & {\color[HTML]{036400} $\uparrow$ 15.1\%}        & {\color[HTML]{036400} $\uparrow$ 1.8\%} & {\color[HTML]{036400} $\uparrow$ 2.9\%} & {\color[HTML]{036400} $\uparrow$ 3.6\%} &  & {\color[HTML]{036400} $\uparrow$ 0.9\%}          & {\color[HTML]{036400} $\uparrow$ 0.6\%}          & {\color[HTML]{036400} $\uparrow$ 0.6\%}          & {\color[HTML]{036400} $\uparrow$ 10.7\%} & {\color[HTML]{036400} $\uparrow$ 10.3\%} & {\color[HTML]{036400} $\uparrow$ 7.52\%} \\
\hline
\end{tabular}%
}
\captionsetup{justification=centering}
\caption{Mean, std-dev of 5 runs for Implicit Emotion Classification in Sarcastic Utterance(Multiclass) on MUStARD++ in a speaker dependent setting}
\label{tab:implicit-Emotion distribution in Sarcastic Utterances-multiclass-speaker-dependent}
\end{table*}

%%%%% Apoorva's results

\begin{table*}[h!]
% \small
\centering
% \resizebox{\textwidth}{!}
{%
\begin{tabular}{c|ccc|ccc|}
\cline{2-7}
\multicolumn{1}{l|}{}                & \multicolumn{6}{c|}{\textbf{Speaker Independent}}                                                                                      \\ \cline{2-7} 
\multicolumn{1}{l|}{}                & \multicolumn{3}{c|}{\textbf{w/o Context}}     & \multicolumn{3}{c|}{\textbf{w Context}}       \\ \cline{2-7}  
\multicolumn{1}{l|}{}                & \textbf{P}    & \textbf{R}    & \textbf{F1}   & \textbf{P}    & \textbf{R}    & \textbf{F1}   \\ \cline{1-7} 
\multicolumn{1}{|c|}{\textbf{T}}     & 40$\pm$0.33          & 40.67$\pm$0.39          & \textcolor{red}{40.3$\pm$0.35}          & 40.3$\pm$0.56          & 41$\pm$0.5          & \textcolor{red}{40.63+-0.52}          \\
\multicolumn{1}{|c|}{\textbf{A}}     & 27.37$\pm$0.81          & 27.85$\pm$2.30          & 27.24$\pm$1.25         & 27.55$\pm$1.59         & 27.62$\pm$1.72          & 27.17$\pm$1.21           \\
\multicolumn{1}{|c|}{\textbf{V}}     & 25.28$\pm$0.87          & 26.06$\pm$1.06         & 25.63$\pm$0.93         & 25.4$\pm$0.45          & 26.19$\pm$0.56         & 25.74$\pm$0.52           \\
\multicolumn{1}{|c|}{\textbf{T+A}}   & 38.73$\pm$1.02          & 39.2$\pm$0.83          & 38.93$\pm$0.92          & 39.1$\pm$0.58          & 39.3$\pm$0.5          & 39.17$\pm$0.53         \\
\multicolumn{1}{|c|}{\textbf{A+V}}   & 25.90$\pm$0.85          & 25.96$\pm$0.8          & 25.9$\pm$0.81          & 25.68$\pm$1.22          & 25.62$\pm$1.33          & 25.62$\pm$1.27          \\
\multicolumn{1}{|c|}{\textbf{V+T}}   & 39.88$\pm$0.48 & 40.47$\pm$0.31 & 40.13$\pm$0.38 & 40.10$\pm$0.8 & 40.8$\pm$0.94 & 40.4$\pm$0.88 \\
\multicolumn{1}{|c|}{\textbf{T+A+V}} & 37.92$\pm$0.89          & 38.27$\pm$0.96          & 38.04$\pm$0.9          & 38.5$\pm$0.98          & 39.0$\pm$1.16          & 38.72$\pm$1.07                 \\ \cline{1-7}  
% \multicolumn{1}{|l|}{\textbf{$\Delta_{multi - unimodel}$}}            & {\color[HTML]{036400} $\uparrow$ 6.2} & {\color[HTML]{036400} $\uparrow$ 9.8} & {\color[HTML]{036400} $\uparrow$ 7.4}        & {\color[HTML]{036400} $\uparrow$ 8.0} & {\color[HTML]{036400} $\uparrow$ 6.5} & {\color[HTML]{036400} $\uparrow$ 7.5} &  & {\color[HTML]{036400} $\uparrow$ 0.7} & {\color[HTML]{036400} $\uparrow$ 4.3} & {\color[HTML]{036400} $\uparrow$ 4.1} & {\color[HTML]{036400} $\uparrow$ 3.7}          & {\color[HTML]{036400} $\uparrow$ 2.7}          & {\color[HTML]{036400} $\uparrow$ 3.4}          \\
% \multicolumn{1}{|l|}{\textbf{\%$\Delta$Unimodal}}           & {\color[HTML]{036400} $\uparrow$ 19.6\%} & {\color[HTML]{036400} $\uparrow$ 31.8\%} & {\color[HTML]{036400} $\uparrow$ 23.7\%}        & {\color[HTML]{036400} $\uparrow$ 23.5\%} & {\color[HTML]{036400} $\uparrow$ 17.1\%} & {\color[HTML]{036400} $\uparrow$ 21.2\%} &  & {\color[HTML]{036400} $\uparrow$ 1.9\%}          & {\color[HTML]{036400} $\uparrow$ 12.6\%}          & {\color[HTML]{036400} $\uparrow$ 12.3\%}          & {\color[HTML]{036400} $\uparrow$ 11.1\%} & {\color[HTML]{036400} $\uparrow$ 7.4\%} & {\color[HTML]{036400} $\uparrow$ 9.9\%} \\ 
\hline
\end{tabular}%
}
\captionsetup{justification=centering}
\caption{Mean, std-dev of 5 runs for Explicit Emotion Classification in Sarcastic Utterance(Multiclass) on MUStARD++ in a speaker independent setting}
\label{tab:explicit-Emotion distribution in Sarcastic Utterances-multiclass-speaker-independent}
\end{table*}

%%%%%%%%%%%%%%%%%%%%%%%%%%%%%%%%%%%%%%%%%%%%%%%%%%%%%%%%%%%%
%%%%% Apoorva's results

\begin{table*}[!ht]
% \small
\centering

% \resizebox{\textwidth}{!}
{%
\begin{tabular}{|c|ccc|ccc|}
\cline{2-7}
\multicolumn{1}{l|}{}                & \multicolumn{6}{c|}{\textbf{Speaker Dependent}}                                               \\ \cline{2-7} 
\multicolumn{1}{l|}{}                & \multicolumn{3}{c|}{\textbf{w/o Context}}     & \multicolumn{3}{c|}{\textbf{w Context}}     \\ \cline{2-7}  
\multicolumn{1}{l|}{}                & \textbf{P}    & \textbf{R}    & \textbf{F1}   & \textbf{P}    & \textbf{R}    & \textbf{F1}   \\ \cline{1-7}  
\multicolumn{1}{|c|}{\textbf{T}}     & 39.33$\pm$0.79          & 40.33$\pm$0.57          & 39.81$\pm$0.69          & 39.5$\pm$0.71          & 40.27$\pm$0.82          & 39.89$\pm$0.76          \\
\multicolumn{1}{|c|}{\textbf{A}}     & 28.38$\pm$0.99          & 30.92$\pm$0.69          & 29.32$\pm$0.87          & 28.28$\pm$1.52          & 27.15$\pm$3.18          & 27.25$\pm$2.01         \\
\multicolumn{1}{|c|}{\textbf{V}}     & 26.97$\pm$1.09          & 36.67$\pm$0.93          & 28.27$\pm$0.71          & 29.21$\pm$0.8          & 35.44$\pm$0.46          & 30.34$\pm$0.41         \\
\multicolumn{1}{|c|}{\textbf{T+A}}   & 39.76$\pm$0.7          & 40.13$\pm$0.83          & 39.9$\pm$0.73          & 40.17$\pm$0.77          & 40.6$\pm$0.76          & \textcolor{red}{40.36$\pm$0.76}          \\
\multicolumn{1}{|c|}{\textbf{A+V}}   & 27.78$\pm$1.08          & 28.02$\pm$1.66          & 27.85$\pm$1.35          & 28.33$\pm$0.77          & 28.75$\pm$0.78          & 28.52$\pm$0.77          \\
\multicolumn{1}{|c|}{\textbf{V+T}}   & 39.85$\pm$0.66 & 40$\pm$0.52 & 39.91$\pm$0.58 & 39.08$\pm$0.77 & 39.4$\pm$0.78 & 39.23$\pm$0.77 \\
\multicolumn{1}{|c|}{\textbf{T+A+V}} &40.15$\pm$0.68          & 39.8$\pm$0.77          & \textcolor{red}{39.93$\pm$0.72}          & 40.56$\pm$0.48          & 39.97$\pm$0.41          & 40.21$\pm$0.44          \\ \cline{1-7}
% \multicolumn{1}{|l|}{\textbf{$\Delta_{multi - unimodel}$}}            & {\color[HTML]{036400} $\uparrow$ 6.2} & {\color[HTML]{036400} $\uparrow$ 9.8} & {\color[HTML]{036400} $\uparrow$ 7.4}        & {\color[HTML]{036400} $\uparrow$ 8.0} & {\color[HTML]{036400} $\uparrow$ 6.5} & {\color[HTML]{036400} $\uparrow$ 7.5} &  & {\color[HTML]{036400} $\uparrow$ 0.7} & {\color[HTML]{036400} $\uparrow$ 4.3} & {\color[HTML]{036400} $\uparrow$ 4.1} & {\color[HTML]{036400} $\uparrow$ 3.7}          & {\color[HTML]{036400} $\uparrow$ 2.7}          & {\color[HTML]{036400} $\uparrow$ 3.4}          \\
% \multicolumn{1}{|l|}{\textbf{\%$\Delta$Unimodal}}           & {\color[HTML]{036400} $\uparrow$ 19.6\%} & {\color[HTML]{036400} $\uparrow$ 31.8\%} & {\color[HTML]{036400} $\uparrow$ 23.7\%}        & {\color[HTML]{036400} $\uparrow$ 23.5\%} & {\color[HTML]{036400} $\uparrow$ 17.1\%} & {\color[HTML]{036400} $\uparrow$ 21.2\%} &  & {\color[HTML]{036400} $\uparrow$ 1.9\%}          & {\color[HTML]{036400} $\uparrow$ 12.6\%}          & {\color[HTML]{036400} $\uparrow$ 12.3\%}          & {\color[HTML]{036400} $\uparrow$ 11.1\%} & {\color[HTML]{036400} $\uparrow$ 7.4\%} & {\color[HTML]{036400} $\uparrow$ 9.9\%} \\ 
\hline
\end{tabular}%
}
\captionsetup{justification=centering}
\caption{Mean, std-dev of 5 runs for Explicit Emotion Classification in Sarcastic Utterance(Multiclass) on MUStARD++ in a speaker dependent setting}
\label{tab:explicit-Emotion distribution in Sarcastic Utterances-multiclass-dependent}
\end{table*}

\begin{table}[ht!]
\resizebox{\columnwidth}{!}{%
\begin{tabular}{r|ccc|c|ccc|}
\cline{2-8}
\multicolumn{1}{c|}{\multirow{2}{*}{}}          & \multicolumn{3}{c|}{\textit{\textbf{Implicit}}}                                 & \multirow{7}{*}{\textit{\textbf{}}} & \multicolumn{3}{c|}{\textit{\textbf{Explicit}}}                                 \\ \cline{2-4} \cline{6-8} 
\multicolumn{1}{c|}{}                           & \textbf{P}               & \textbf{R}               & \textbf{F1}               &                                     & \textbf{P}               & \textbf{R}               & \textbf{F1}               \\ \cline{1-4} \cline{6-8} 
\multicolumn{1}{|r|}{\textbf{Majority}}         & 14.1                     & 37.6                     & 20.6                      &                                     & 17.0                     & 41.3                     & 24.1                      \\
\multicolumn{1}{|r|}{\textbf{Random (Uniform)}} & 25.3                     & 20.3                     & 21.4                      &                                     & 27.9                     & 11.8                     & 15.5                      \\
\multicolumn{1}{|r|}{\textbf{Random (Prior)}}   & 25.9                     & 25.9                     & 25.9                      &                                     & 26.1                     & 26.1                     & 26.1                      \\
\multicolumn{1}{|r|}{\textbf{ONEvsREST (w BERT)}}        & \multicolumn{1}{l}{25.9} & \multicolumn{1}{l}{36.4} & \multicolumn{1}{l|}{35.6} &                                     & \multicolumn{1}{l}{40.0}   & \multicolumn{1}{l}{44.2}   & \multicolumn{1}{l|}{42.6}   \\
\multicolumn{1}{|r|}{\textbf{ONEvsREST (w BART)}}        & \multicolumn{1}{l}{36} & \multicolumn{1}{l}{38} & \multicolumn{1}{l|}{37} &                                     & \multicolumn{1}{l}{41.2
}   & \multicolumn{1}{l}{	43.6}   & \multicolumn{1}{l|}{	42.0}   \\                                    & \multicolumn{1}{l}{40.0}   & \multicolumn{1}{l}{44.2}   & \multicolumn{1}{l|}{42.6}   \\
\multicolumn{1}{|r|}{\textbf{MultiClass (w BERT)}}       & \multicolumn{1}{r}{35.3} & \multicolumn{1}{r}{36.6} & \multicolumn{1}{r|}{35.7} &                                     & \multicolumn{1}{r}{42.0} & \multicolumn{1}{r}{44.3} & \multicolumn{1}{r|}{42.8} \\
\multicolumn{1}{|r|}{\textbf{MultiClass (w BART)}}       & \multicolumn{1}{r}{35} & \multicolumn{1}{r}{38} & \multicolumn{1}{r|}{36} &                                     & \multicolumn{1}{r}{41.7} & \multicolumn{1}{r}{44.0} & \multicolumn{1}{r|}{42.6} \\
\hline
\end{tabular}%
    }
    %\captionsetup{justification=centering}
    \caption{Benchmarking emotion classification results comparison across different methods}
    \label{tab:result-comparision}
\end{table}
